# Supplementary material for: TOP: Backdoor Detection in Neural Networks via Transferability of Perturbation
Source: arXiv:2103.10274 source file (2021-03-18)
Supplement: Supplementary file 1 [file appendix.tex]

% \newpage
\clearpage

\begin{center}
{\Large Supplementary Material for \\
\vspace{1mm}
\textbf{TOP: Backdoor Detection in Neural Networks via Transferability of Perturbation}}\\
\vspace{2mm}
\author{Todd Huster, Emmanuel Ekwedike}
\end{center}
 \vspace{2mm}
 
 \section{Deep Neural Networks (DNN) Background}
 \subsection{DNN Training}
 \noindent A DNN is a function that classifies an n-dimensional input $x\in \RR^n$  into one of $k$ classes. The output of the DNN $y\in \RR^k$ is a probability distribution over the $k$ classes. Mathematically, a DNN can be represented by a parameterized function $f_{\btheta}:\RR^n \rightarrow \RR^k$ where $\btheta$ represents the function’s parameters
%  \subsection{DNN Training}
 Let $\cD_{train} =\Big \{(x^{(i)},y^{(i)})\Big \}_{i=1}^m$ denote the training sample set. Where
\begin{align*}
m &: \text{is the number of training samples.}\\
x^{(i)} &: \text{ is the input variable (feature).}\\
y^{(i)} &: \text{is the output variable (target).}
\end{align*}
The parameters of a DNN are determined by training the network on a training dataset $\cD_{train} =\Big \{(x^{(i)},y^{(i)})\Big \}_{i=1}^m$ . 
The total cost for loss over our entire training dataset $\cD_{train} =\Big \{(x^{(i)},y^{(i)})\Big \}_{i=1}^m$ is given by the cost function
\begin{align}
J(\btheta)&=  \frac{1}{m} \sum_{i=1}^m \cL\Big( f_{\btheta}\left(x^{(i)}\right), y^{(i)}\Big)
\end{align}
The training procedure determines parameters  that minimize the average distance, measured using a loss function $\cL$, between the network’s predictions on the training dataset and ground-truth as follows:

\begin{align}
\btheta^{\star}&\in\argmin_{\btheta \in \bTheta}J(\btheta)\nonumber\\
&=\argmin_{\btheta \in \bTheta}\frac{1}{m} \sum_{i=1}^m \cL\Big( f_{\btheta}\left(x^{(i)}\right), y^{(i)}\Big).
\end{align}
 
 \subsection{DNN Architectures in the TrojAI Benchmark Datasets}\label{appedic:section:dnn:arch}
\noindent The network architectures for the TrojAI benchmark datasets are slightly different for each round. Figures \ref{fig:appendix:dnn_arch_r1}, \ref{fig:appendix:dnn_arch_r2}, and \ref{fig:appendix:dnn_arch_r3} show a barplot of model counts in round 1, 2, and 3 respectively. 
\begin{figure}[!htbp]
  \centering
    \includegraphics[width=.45\textwidth]{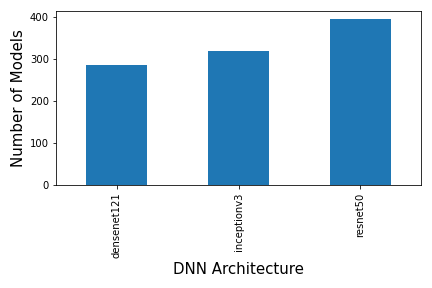} 
    \caption{Bar graph of DNN models architectures in the Round 1 TrojAI dataset}\label{fig:appendix:dnn_arch_r1} 
\end{figure}

\begin{figure}[!htbp]
  \centering
    \includegraphics[width=.45\textwidth]{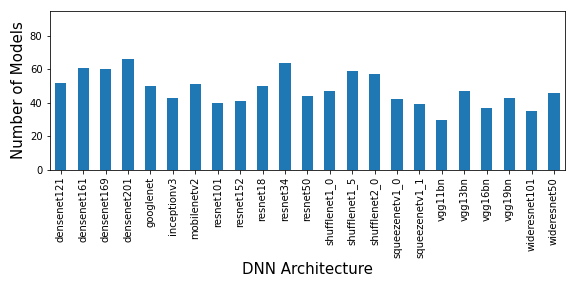} 
    \caption{Bar graph of DNN models architectures in the Round 2 TrojAI dataset}\label{fig:appendix:dnn_arch_r2} 
\end{figure}

\begin{figure}[!htbp]
  \centering
    \includegraphics[width=.45\textwidth]{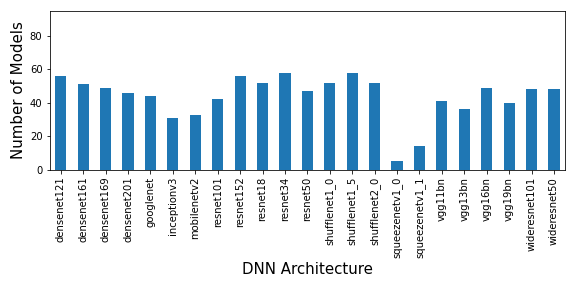} 
    \caption{Bar graph of DNN models architectures in the Round 3 TrojAI dataset}\label{fig:appendix:dnn_arch_r3} 
\end{figure}

 \section{Additional Results}\label{appendix:addtional_results}
We provide additional results of different detectors on the TrojAI round 2 and round 3 datasets.

\begin{figure}[!htbp]
\resizebox{.98\linewidth}{!}{$
\centering
\subfigure[Round 2]{%
\label{fig:r2fc_det1}%
\includegraphics[width=.5\textwidth]{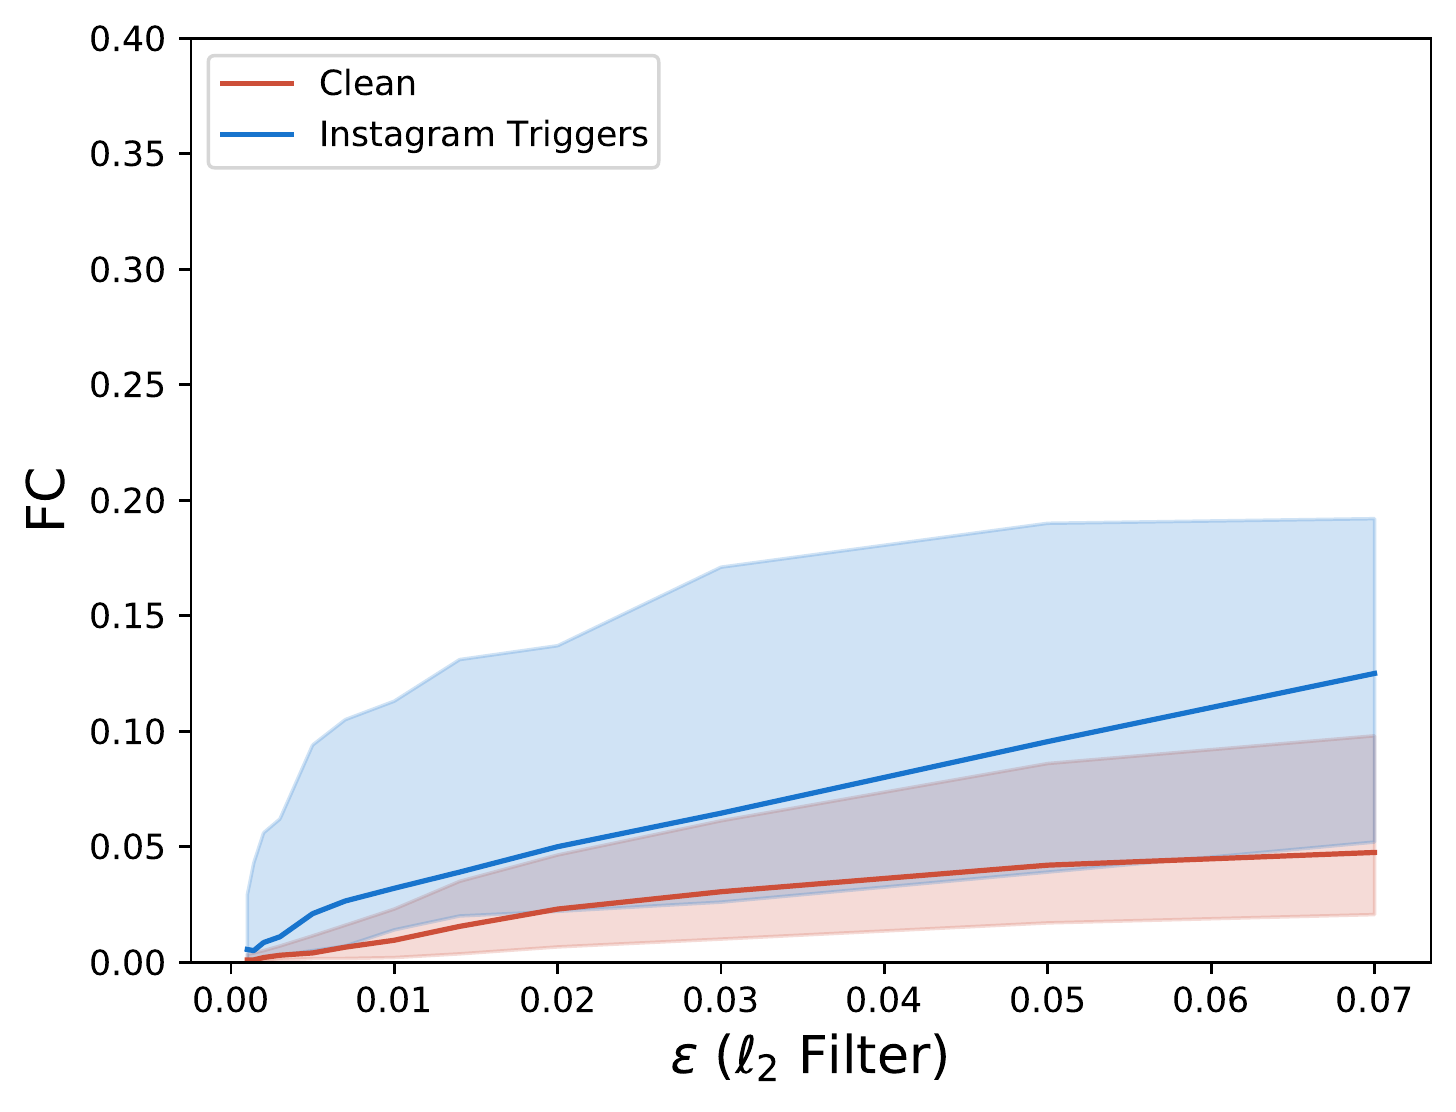}}%
\subfigure[Round 3]{%
\label{fig:r3fc_det1}%
\includegraphics[width=.5\textwidth]{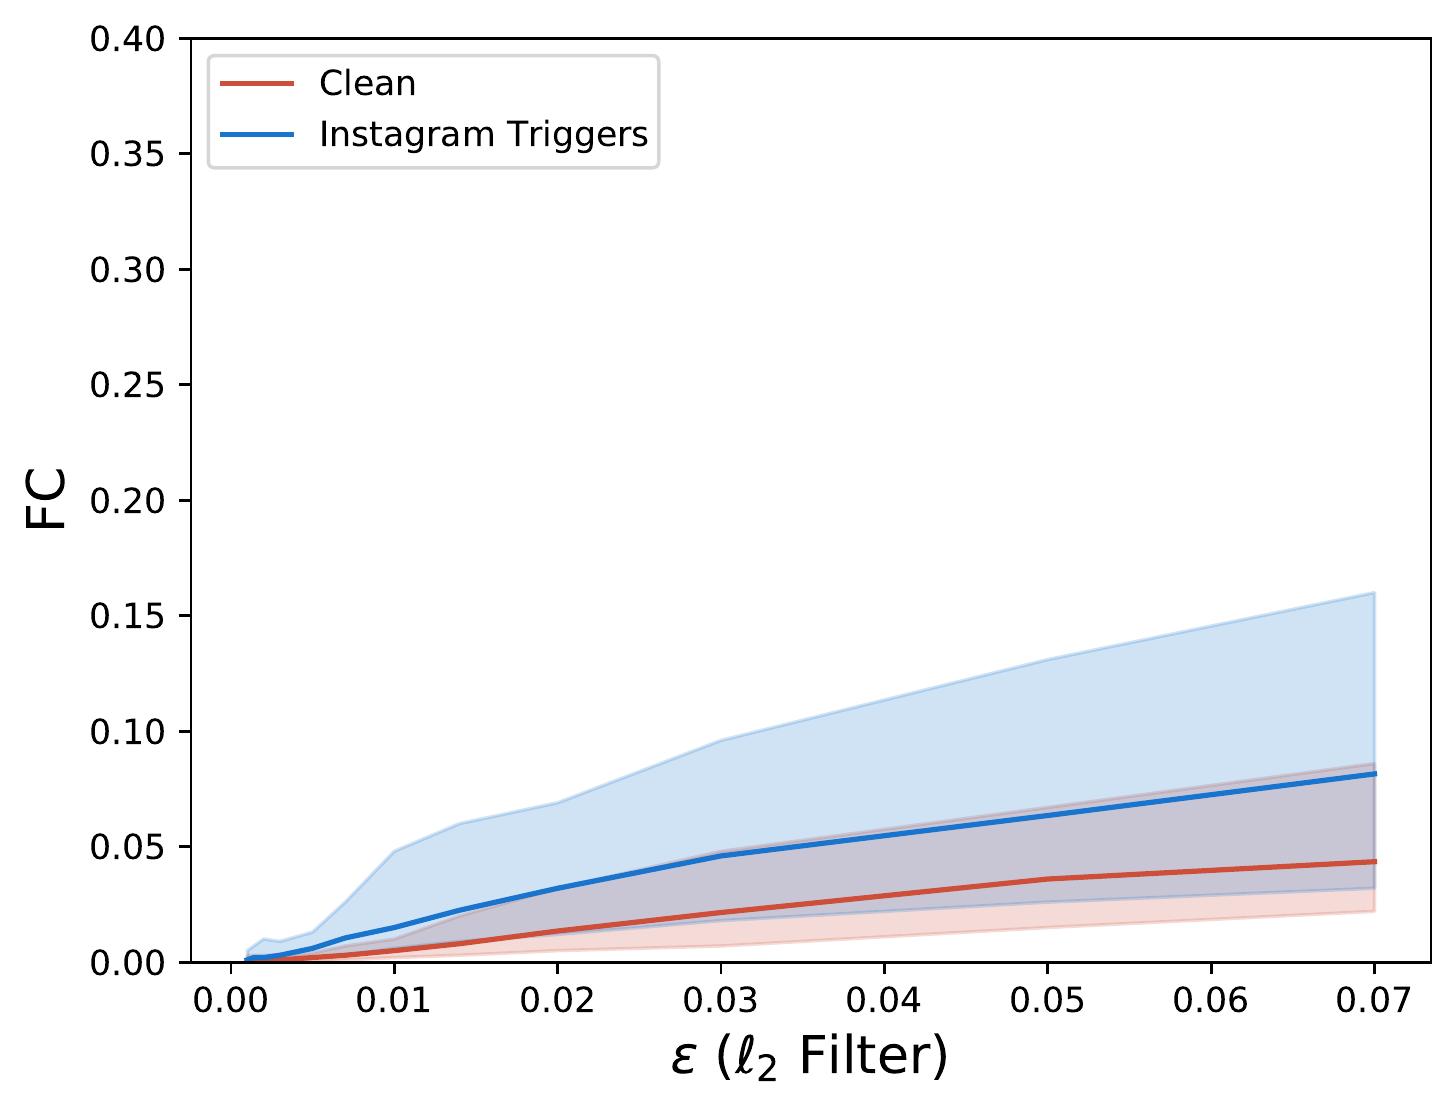}}%
$}
\caption{FC scores for models at different attack strengths}\label{fig:fc_det1}
\end{figure}

\begin{figure}[!htbp]
\resizebox{.98\linewidth}{!}{$ 
\centering
\subfigure[Round 2]{%
\label{fig:r2fc_det2}%
\includegraphics[width=.5\textwidth]{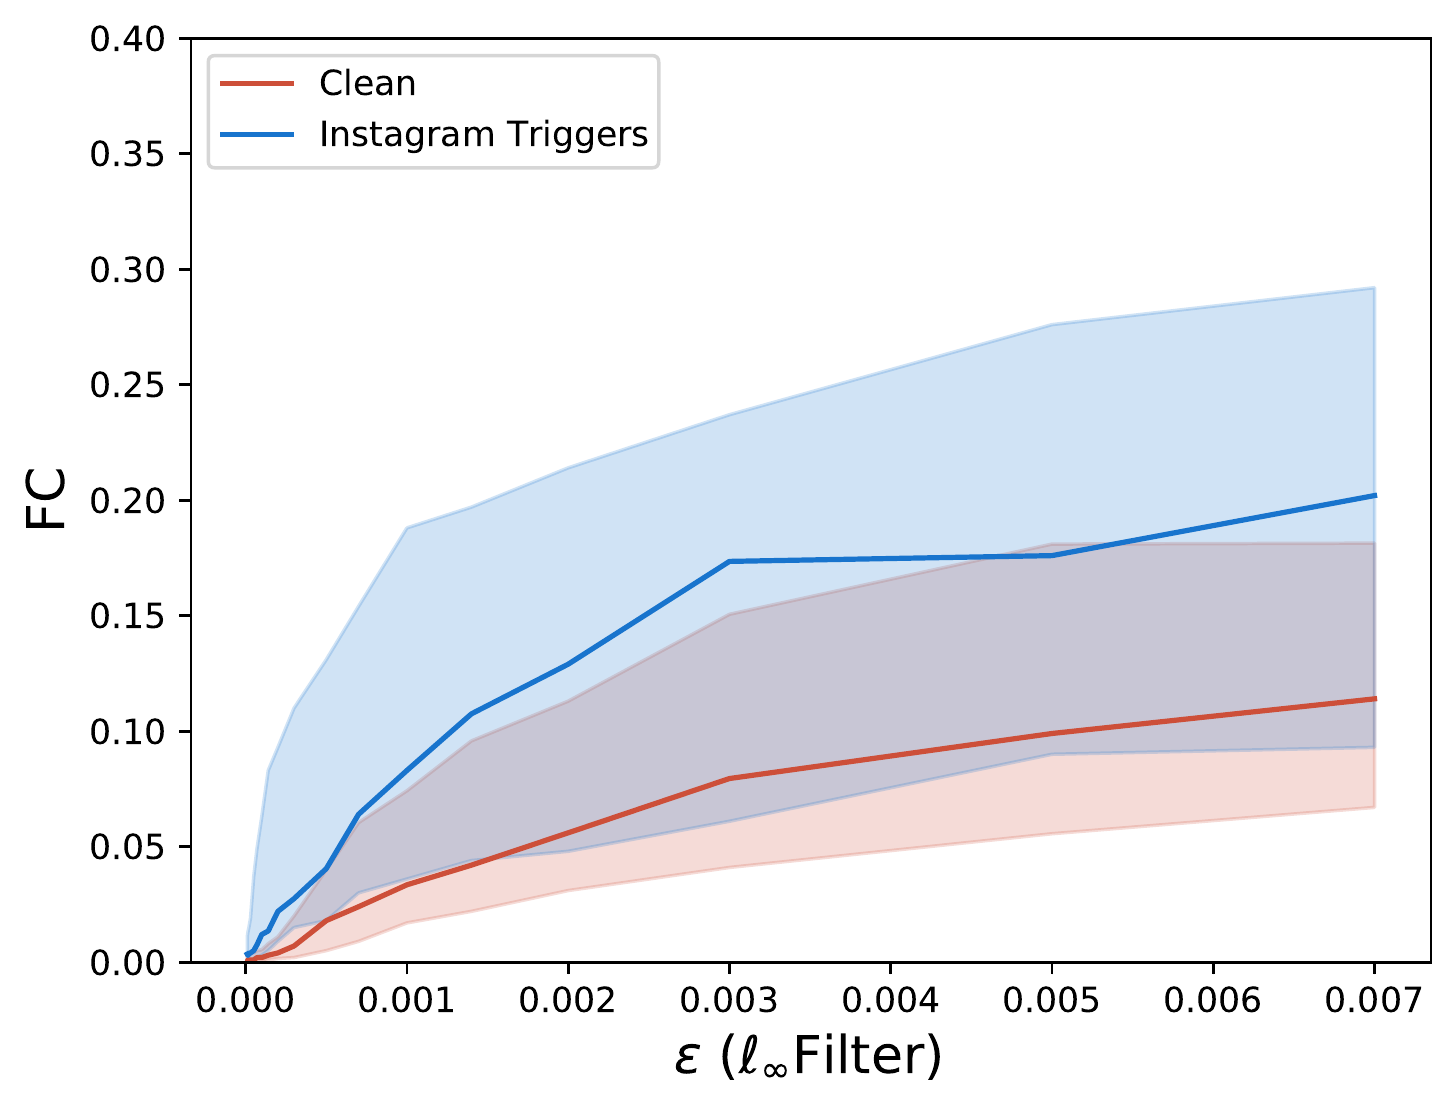}}%
\subfigure[Round 3]{%
\label{fig:r3fc_det2}%
\includegraphics[width=.5\textwidth]{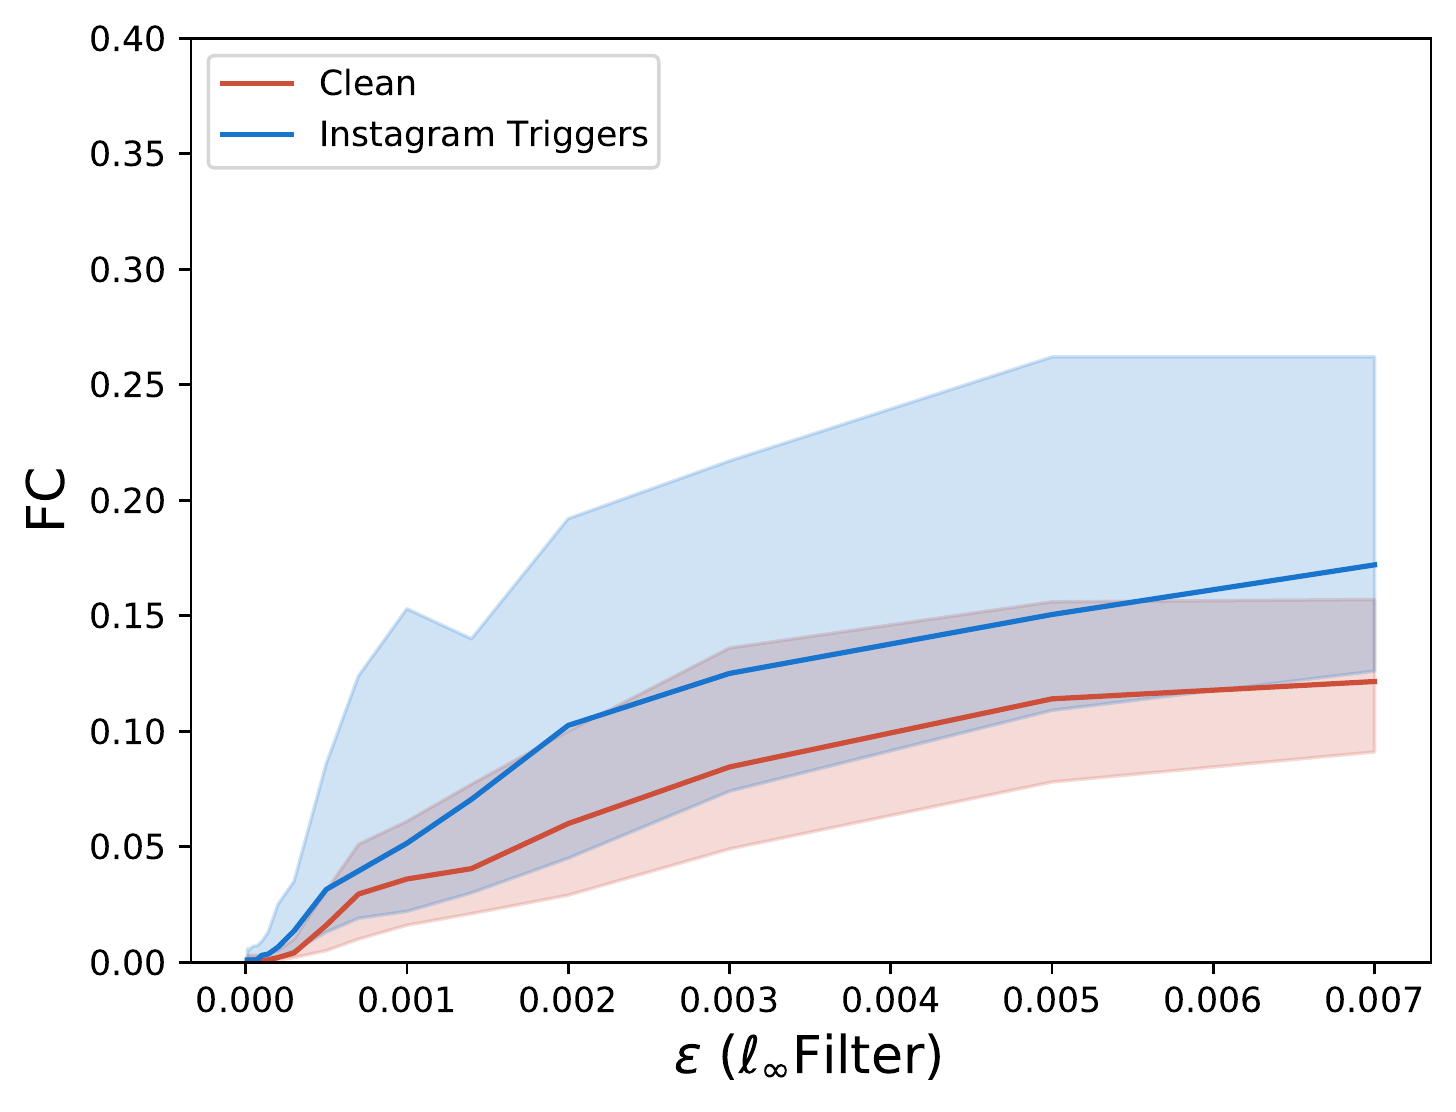}}%
$}
\caption{FC scores for models at different attack strengths}\label{fig:fc_det2}
\end{figure}

Figures \ref{fig:r2fc_det1} and \ref{fig:r3fc_det1} show the median and 80 percentile spread of FC scores, based on $\ell_2$ filter detector, for all attack strengths for rounds 2 and 3 respectively. Figures \ref{fig:r2fc_det2} and \ref{fig:r3fc_det2} show the median and 80 percentile spread of FC scores, based on $\ell_{\infty}$ filter detector, for all attack strengths for rounds 2 and 3 respectively. 

\begin{figure}[!htbp]
\resizebox{.98\linewidth}{!}{$
\centering
\subfigure[Round 2]{%
\label{fig:r2fr_det1}%
\includegraphics[width=.5\textwidth]{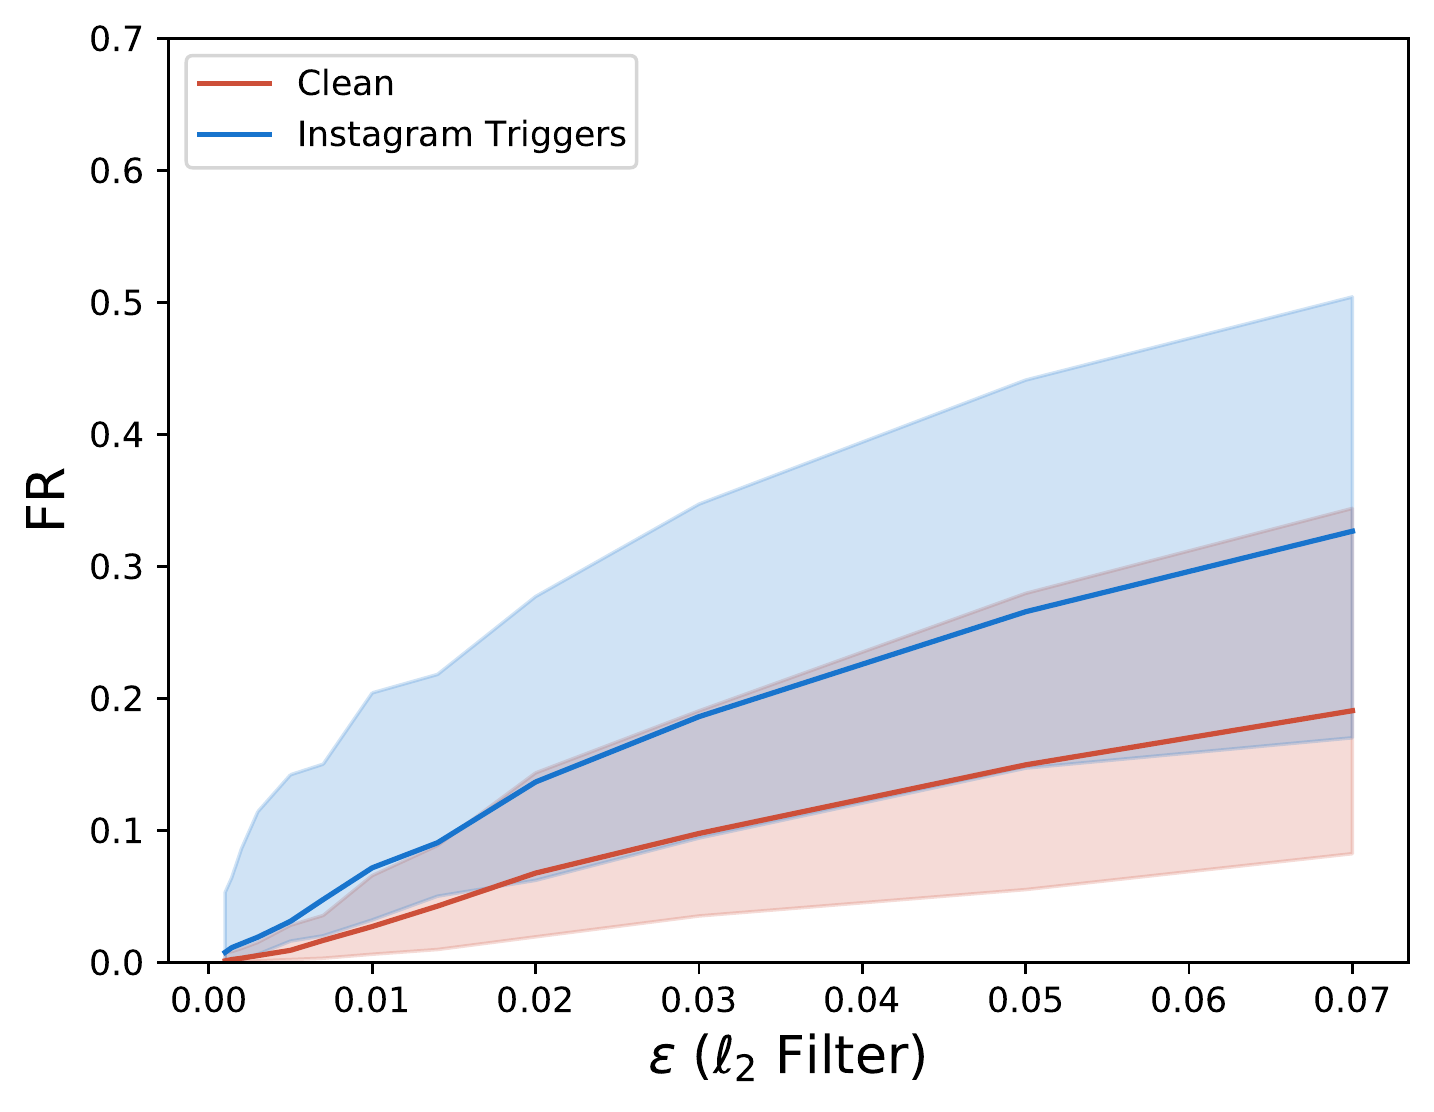}}%
\subfigure[Round 3]{%
\label{fig:r3fr_det1}%
\includegraphics[width=.5\textwidth]{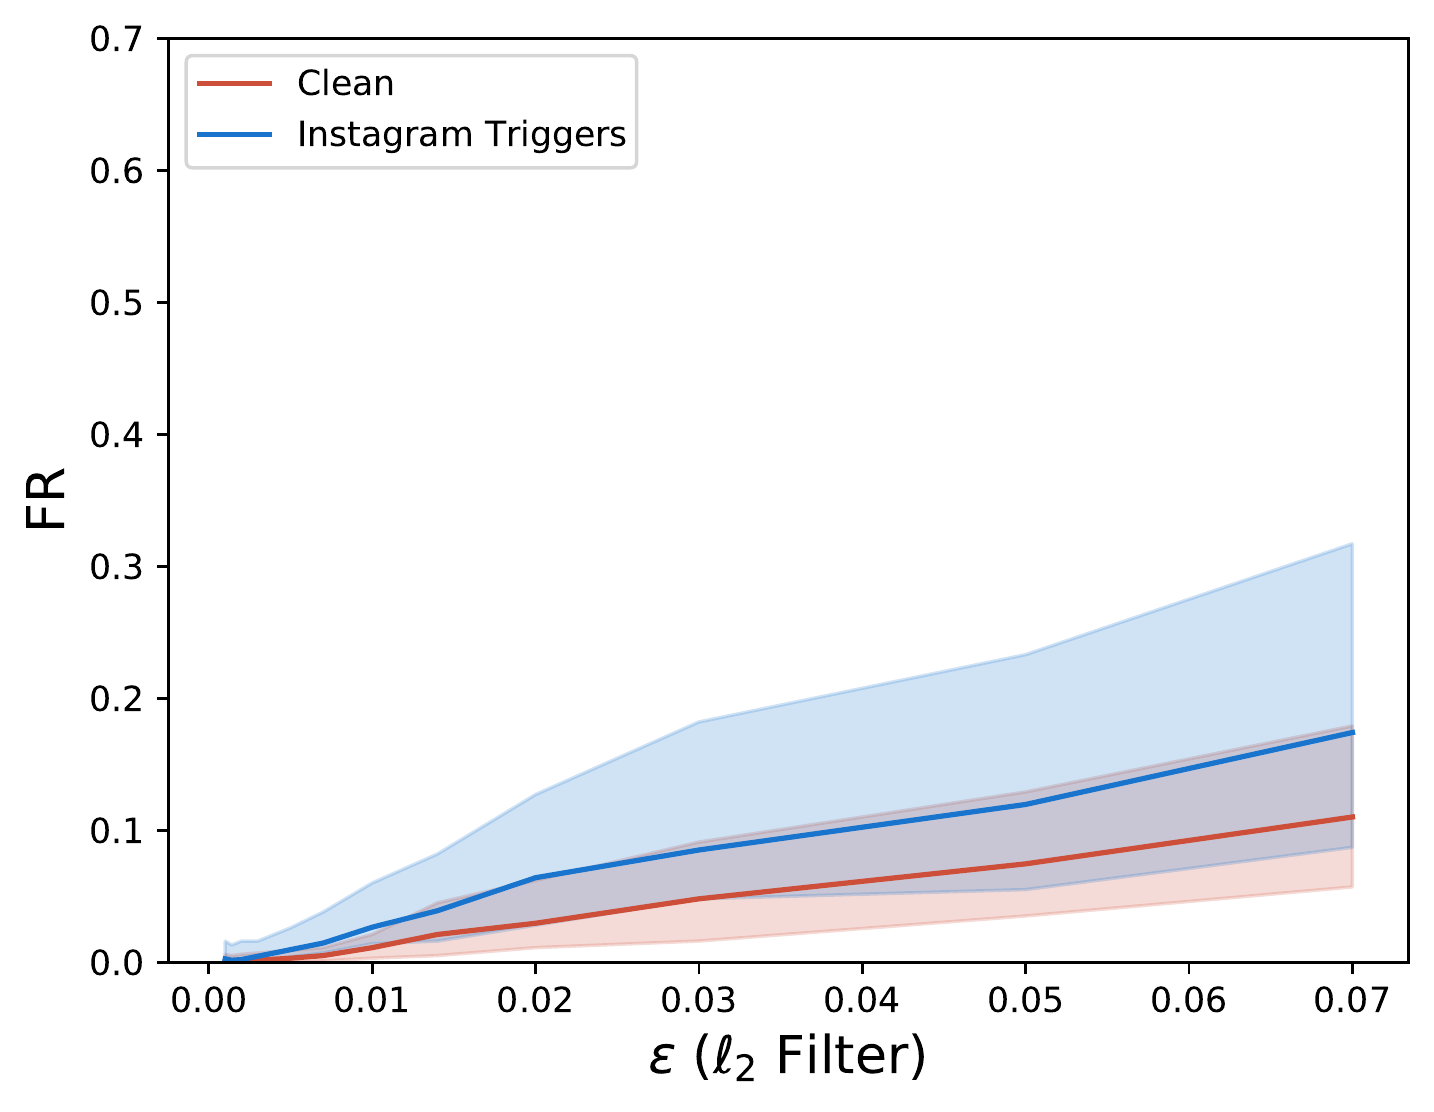}}%
$}
\caption{FR scores for models at different attack strengths}\label{fig:fr_det1}
\end{figure}

\begin{figure}[!htbp]
\resizebox{.98\linewidth}{!}{$
\centering
\subfigure[Round 2]{%
\label{fig:r2fr_det2}%
\includegraphics[width=.5\textwidth]{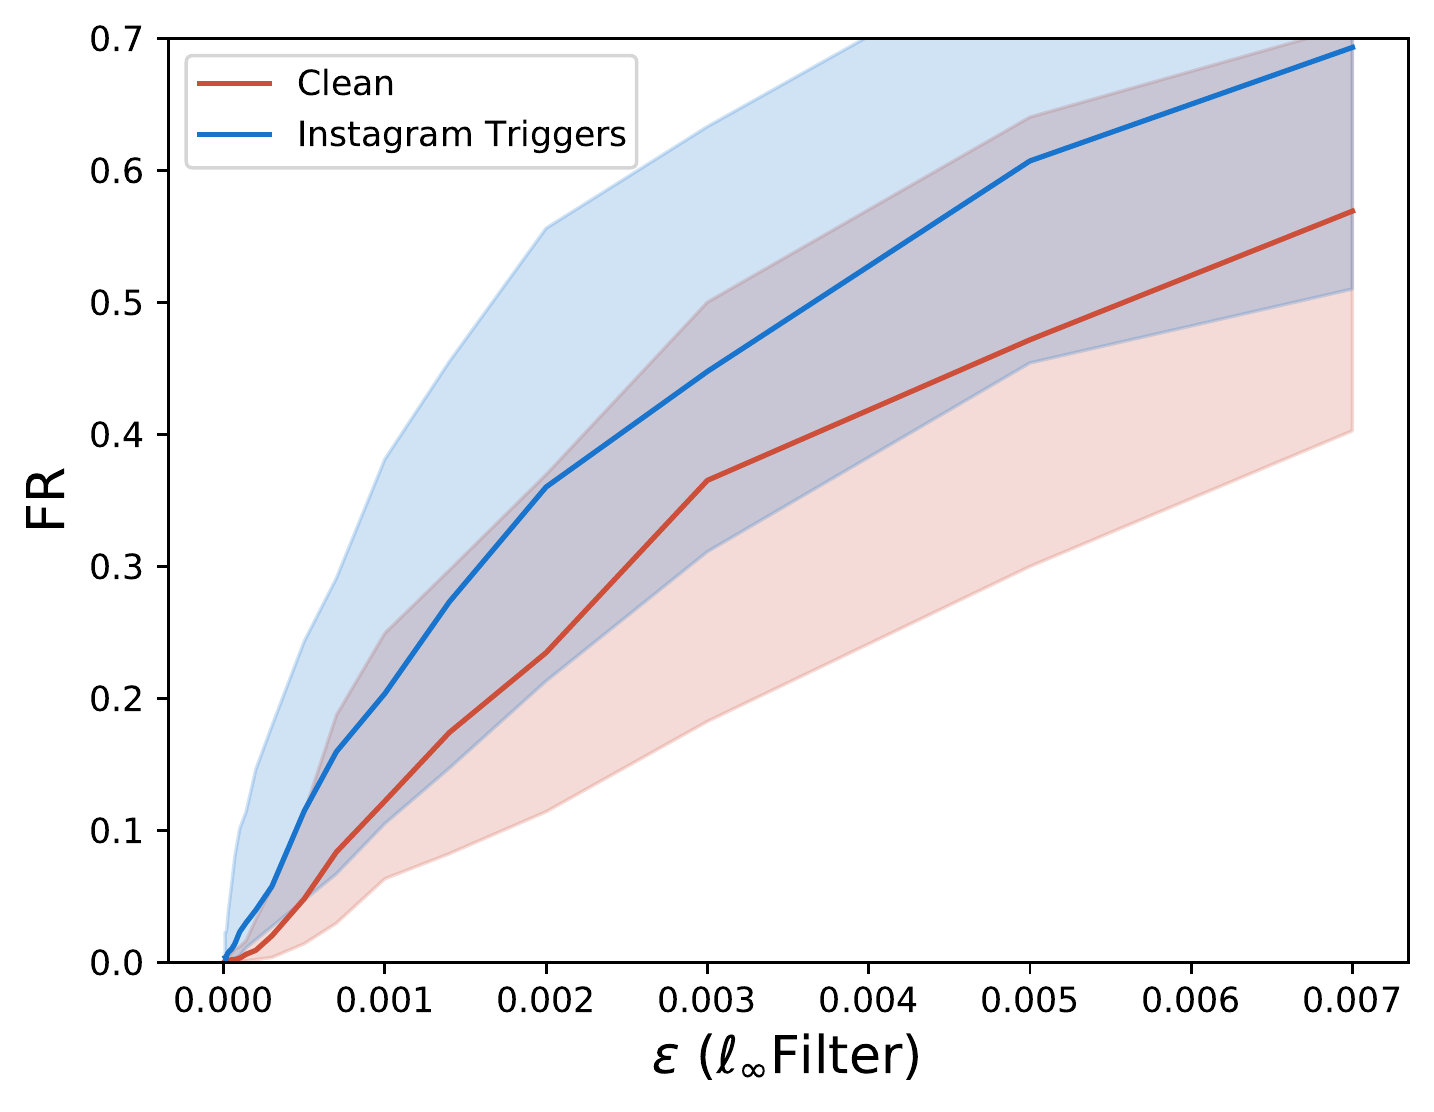}}%
\subfigure[Round 3]{%
\label{fig:r3fr_det2}%
\includegraphics[width=.5\textwidth]{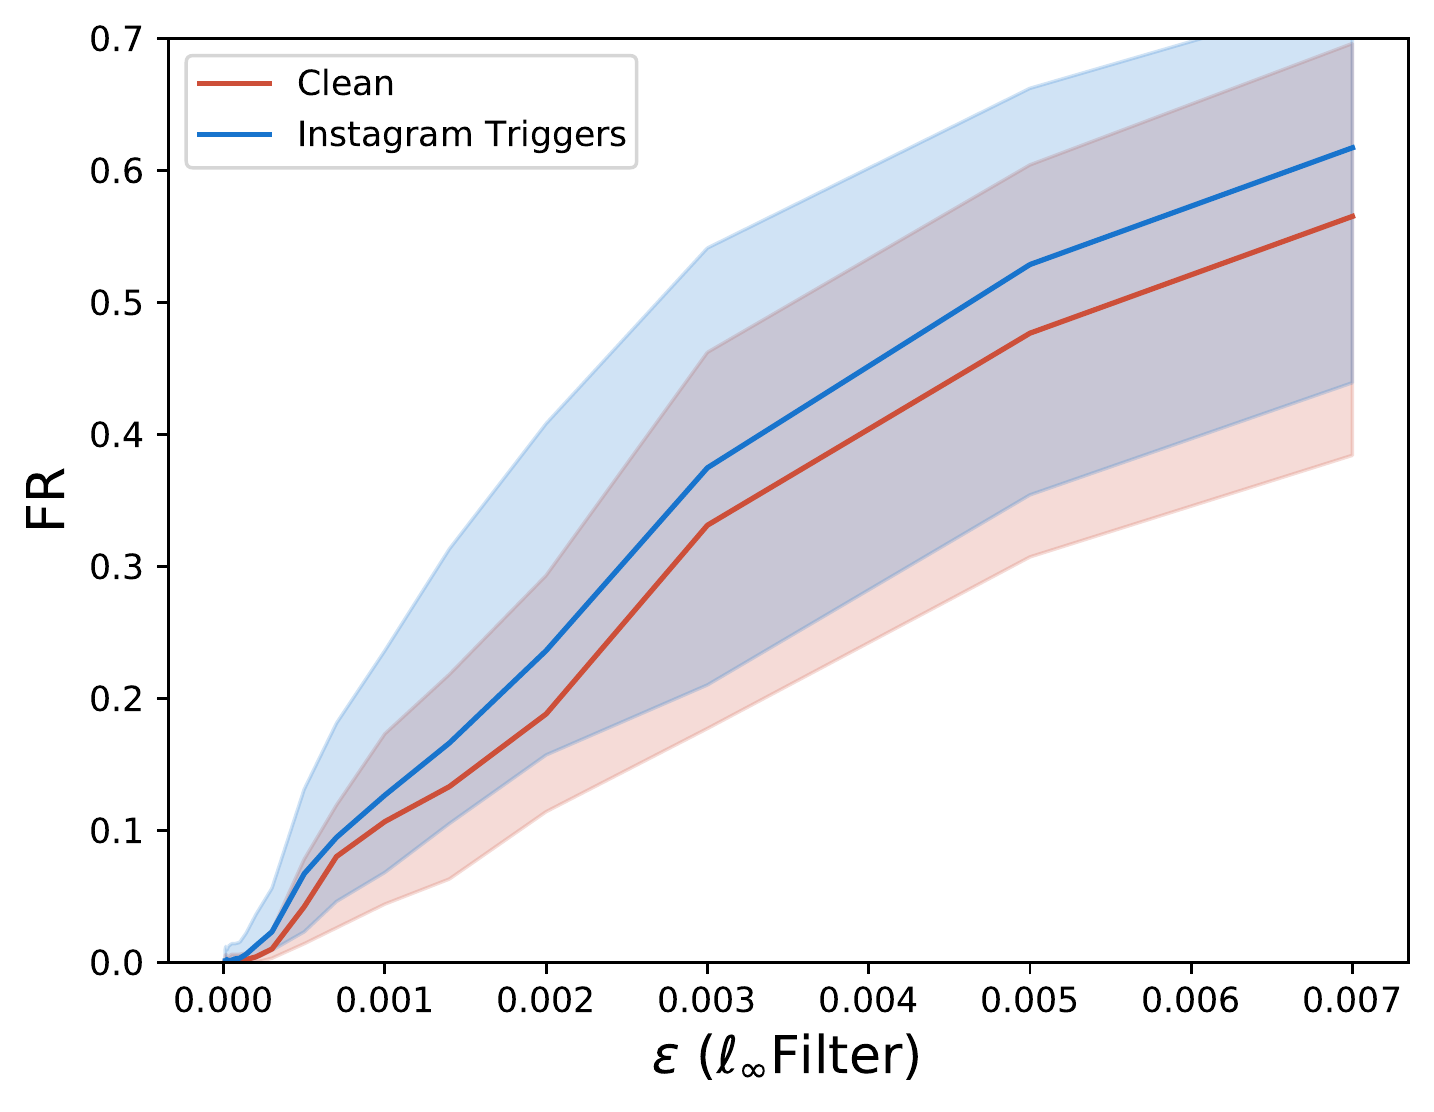}}%
$ }
\caption{FR scores for models at different attack strengths}\label{fig:fr_det2}
\end{figure}

Similarly, Figures \ref{fig:r2fr_det1} and \ref{fig:r3fr_det1} show the median and 80 percentile spread of FR scores, based on $\ell_2$ filter detector, for all attack strengths for rounds 2 and 3 respectively. Figures \ref{fig:r2fr_det2} and \ref{fig:r3fr_det2} show the median and 80 percentile spread of FR scores, based on $\ell_{\infty}$ filter detector, for all attack strengths for rounds 2 and 3 respectively. In what follows, we show experimental results examining how many models are required to calibrate different detectors. We randomly sampled class-balanced subsets of the round 2 and round 3 training set respectively, calibrated different detectors, and evaluated them on the test models. We performed this experiment 200 times for each training set size.  

%%%%%%%%%%%%%
%Detector 1
%%%%%%%%%%%%
\begin{figure}[!htbp]
\resizebox{.98\linewidth}{!}{$
\centering
\subfigure[Round 2]{%
\label{fig:r2auc_det1}%
\includegraphics[width=.5\textwidth]{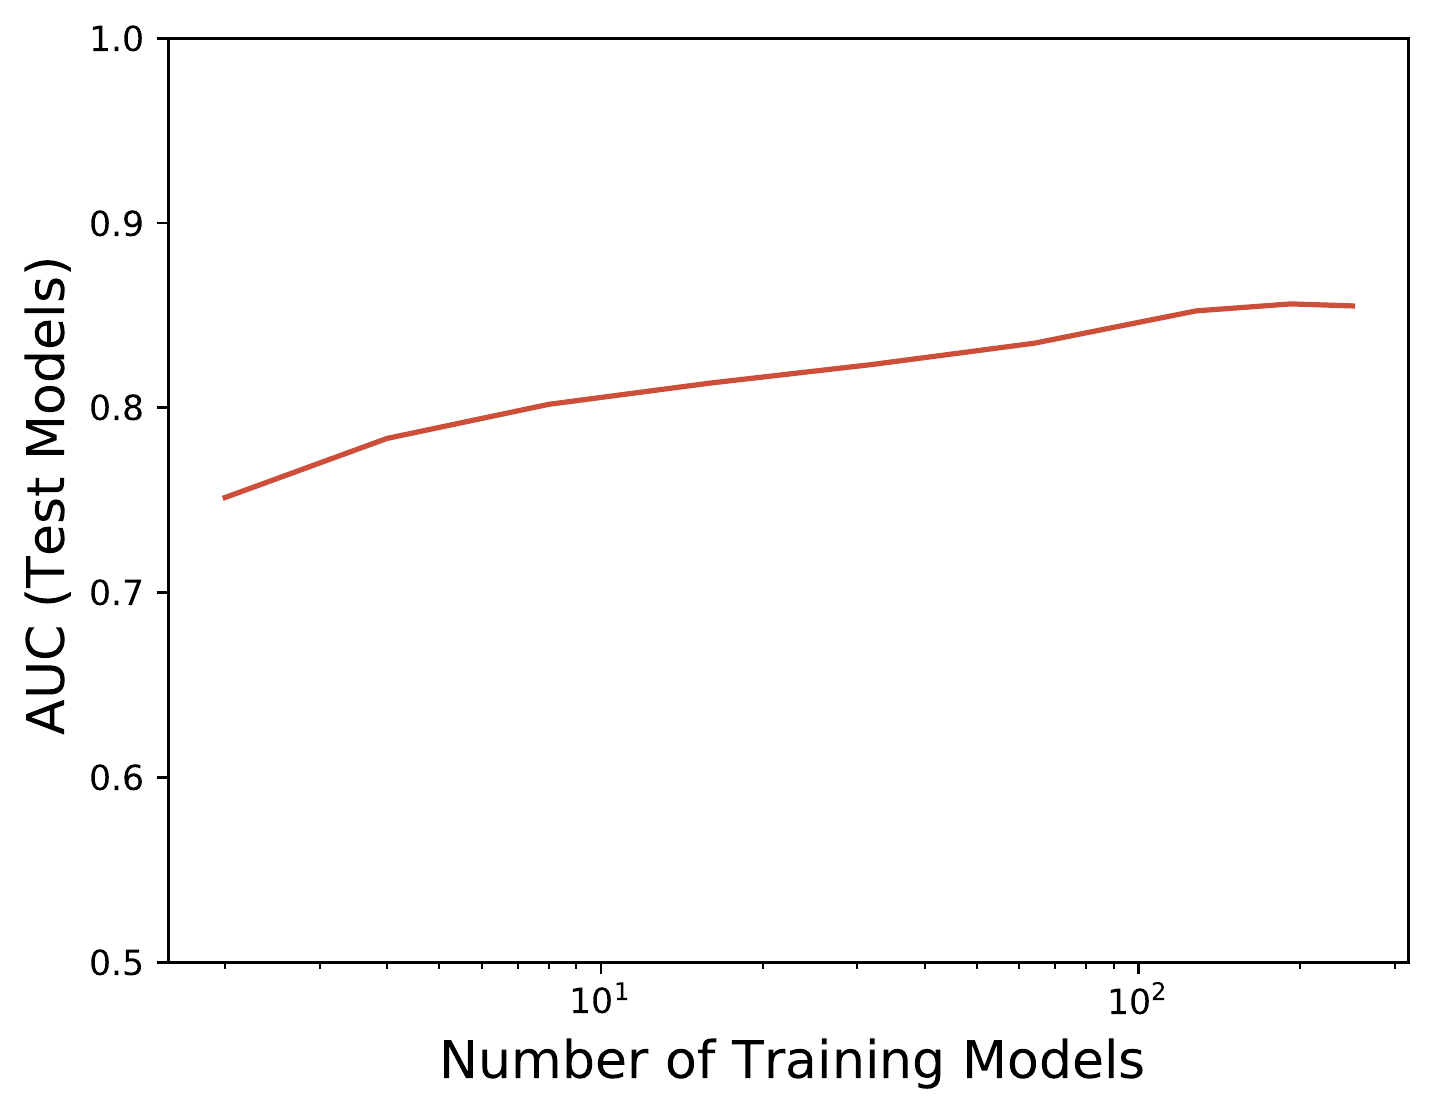}}%
\subfigure[Round 3 ]{%
\label{fig:r3auc_det1}%
\includegraphics[width=.5\textwidth]{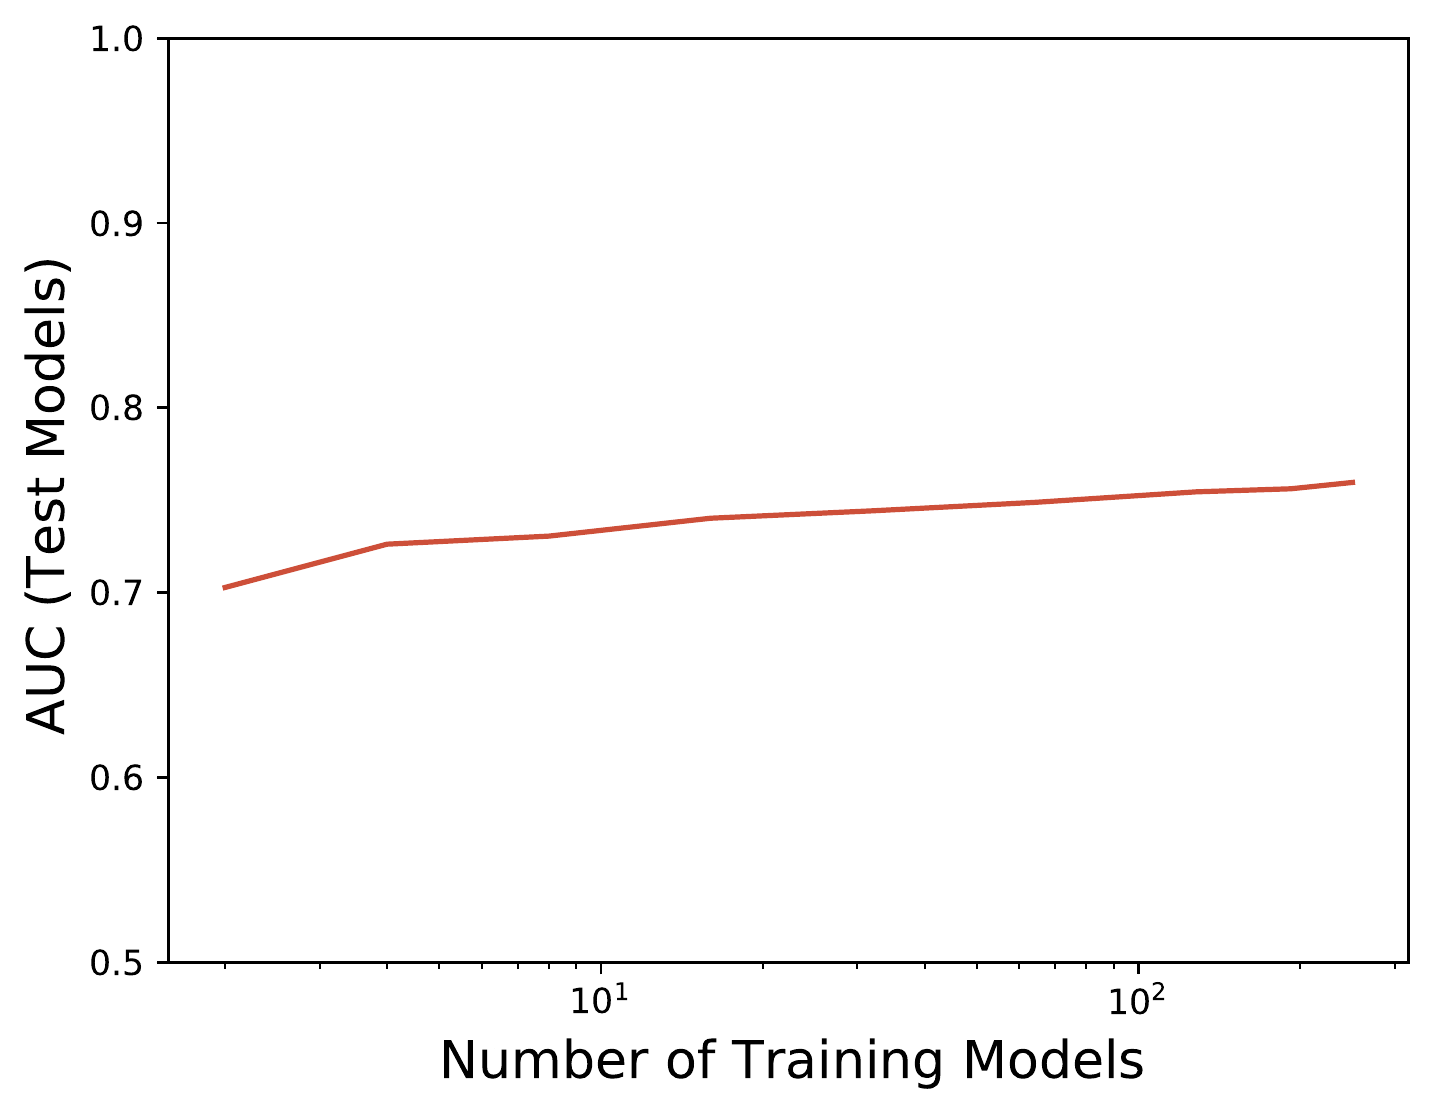}}%
$ }
\caption{The AUC for Instagram vs. None corresponding to $\ell_2$-filter detector}
\end{figure}

\begin{figure}[!htbp]
\resizebox{.98\linewidth}{!}{$
\centering
\subfigure[Round 2]{%
\label{fig:r2ce_det1}%
\includegraphics[width=.5\textwidth]{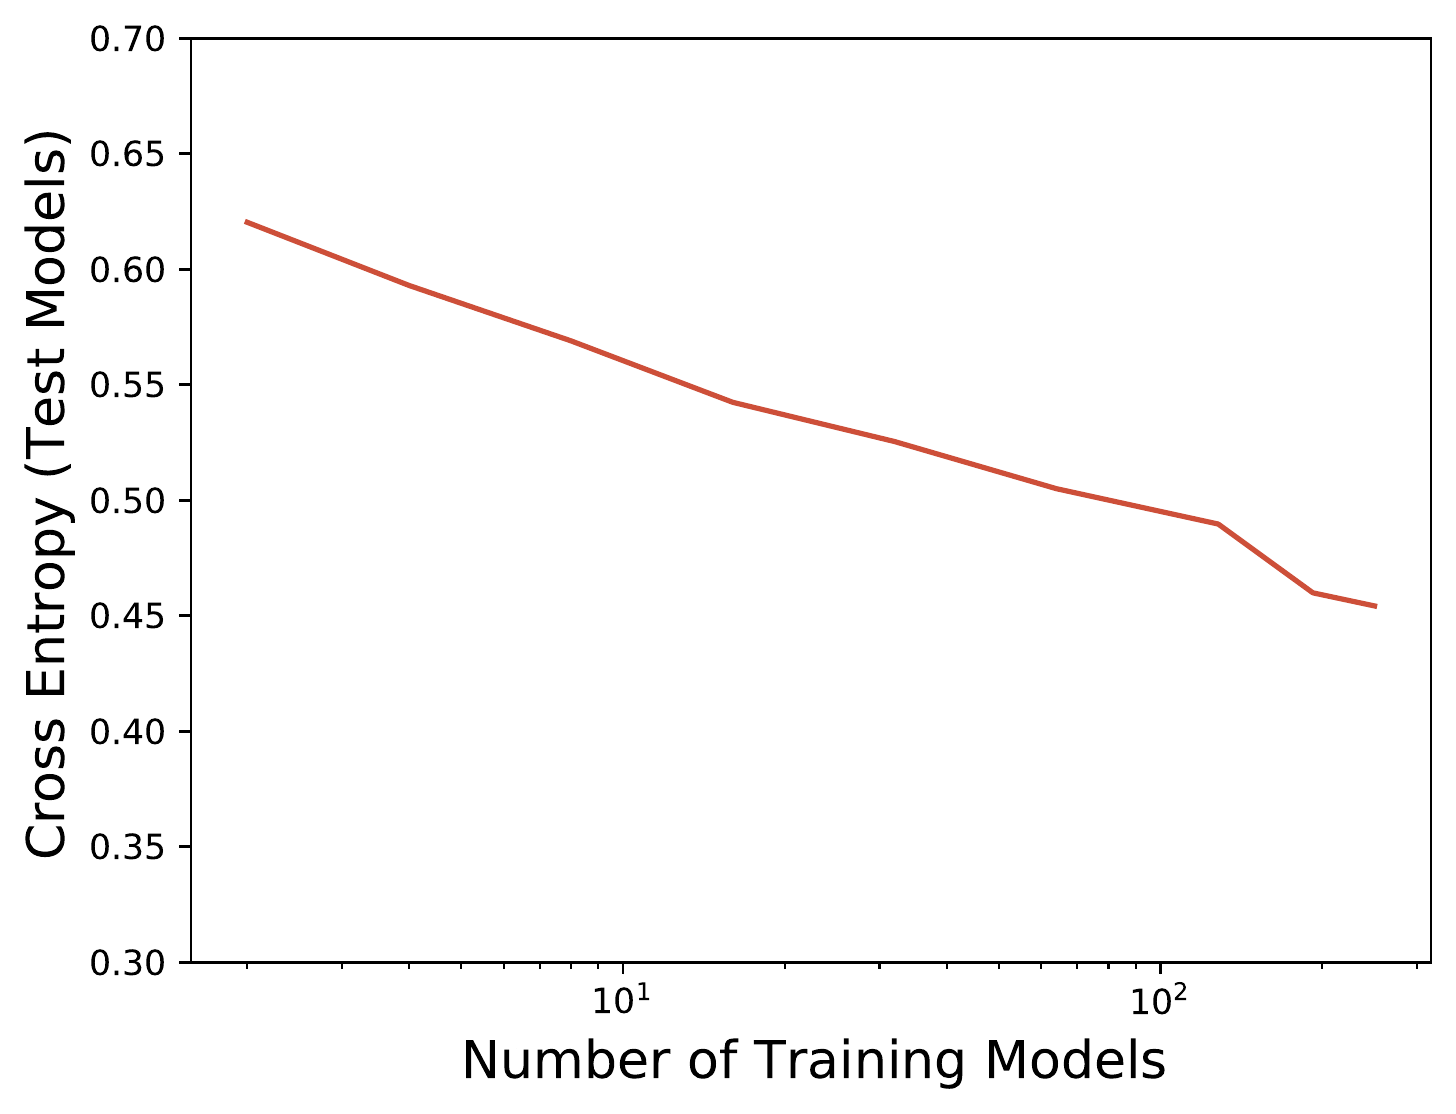}}%
\subfigure[Round 3 ]{%
\label{fig:r3ce_det1}%
\includegraphics[width=.5\textwidth]{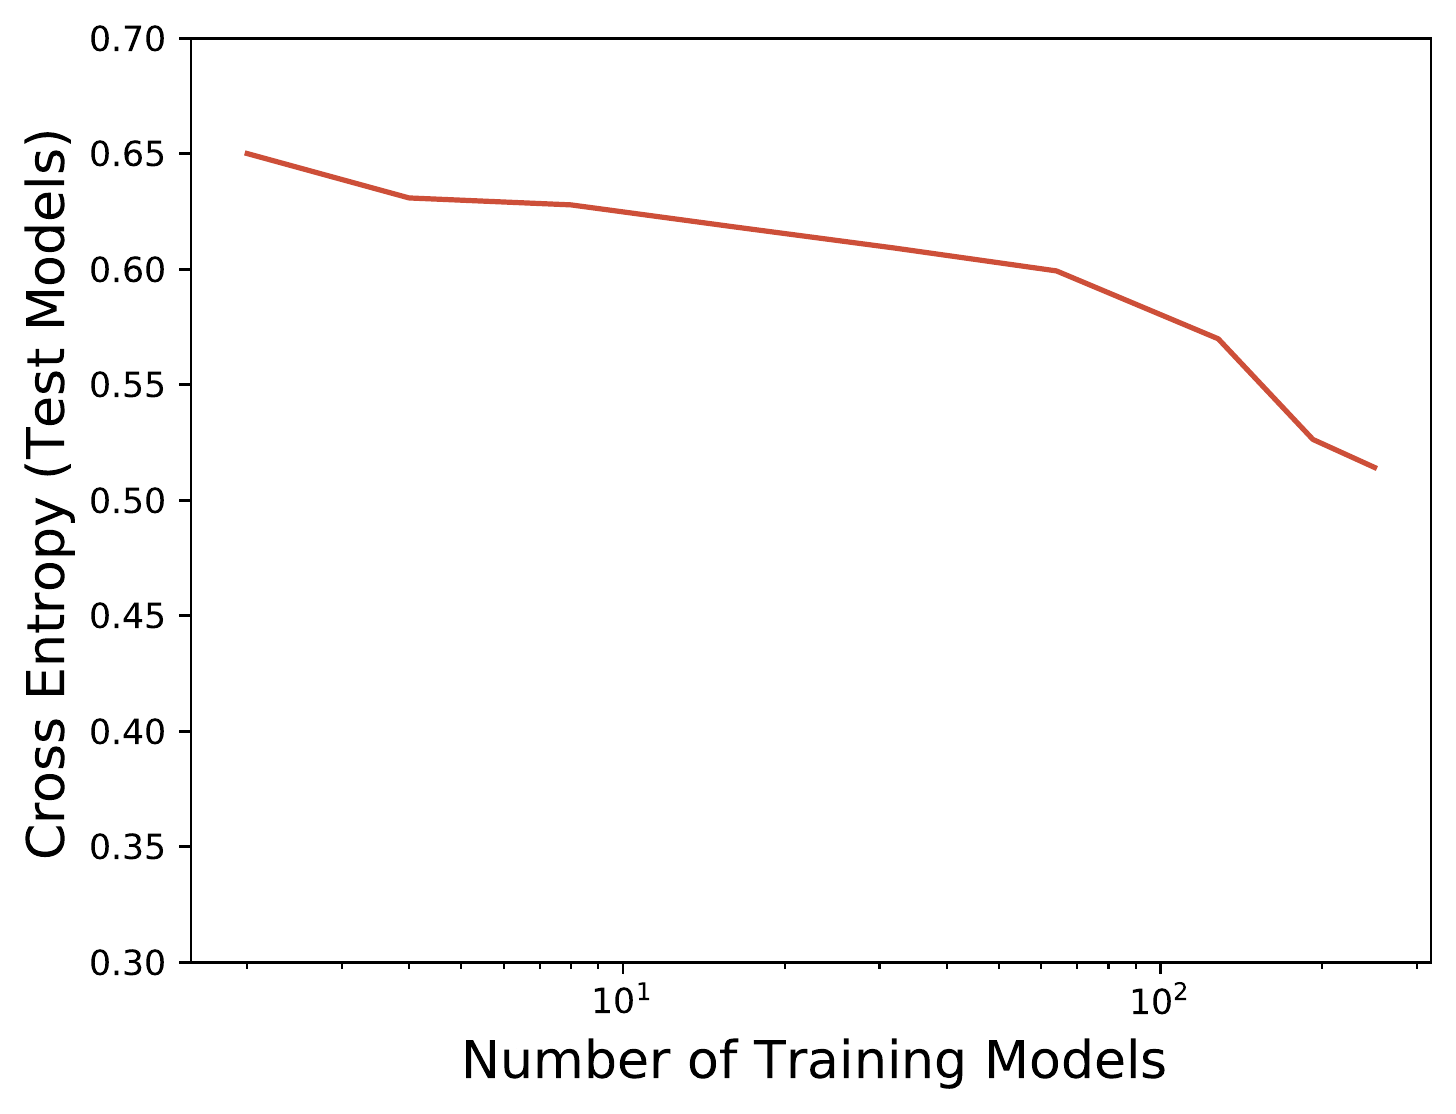}}%
$}
\caption{The CE for Instagram vs. None corresponding to $\ell_2$-filter detector}
\end{figure}
Figures \ref{fig:r2auc_det1} and \ref{fig:r2ce_det1} show how the number of training models impacts the top-level metric, for the $\ell_{2}$ filter detector,  in round 2. Similar, Figures \ref{fig:r3auc_det1} and \ref{fig:r3ce_det1} show how the number of training models impacts the top-level metric, for the $\ell_{2}$ filter detector,  in round 3.

 %%%%%%%%%%%%%
%Detector 2
%%%%%%%%%%%%
\begin{figure}[!htbp]
\resizebox{.98\linewidth}{!}{$
\centering
\subfigure[Round 2]{%
\label{fig:r2auc_det2}%
\includegraphics[width=.5\textwidth]{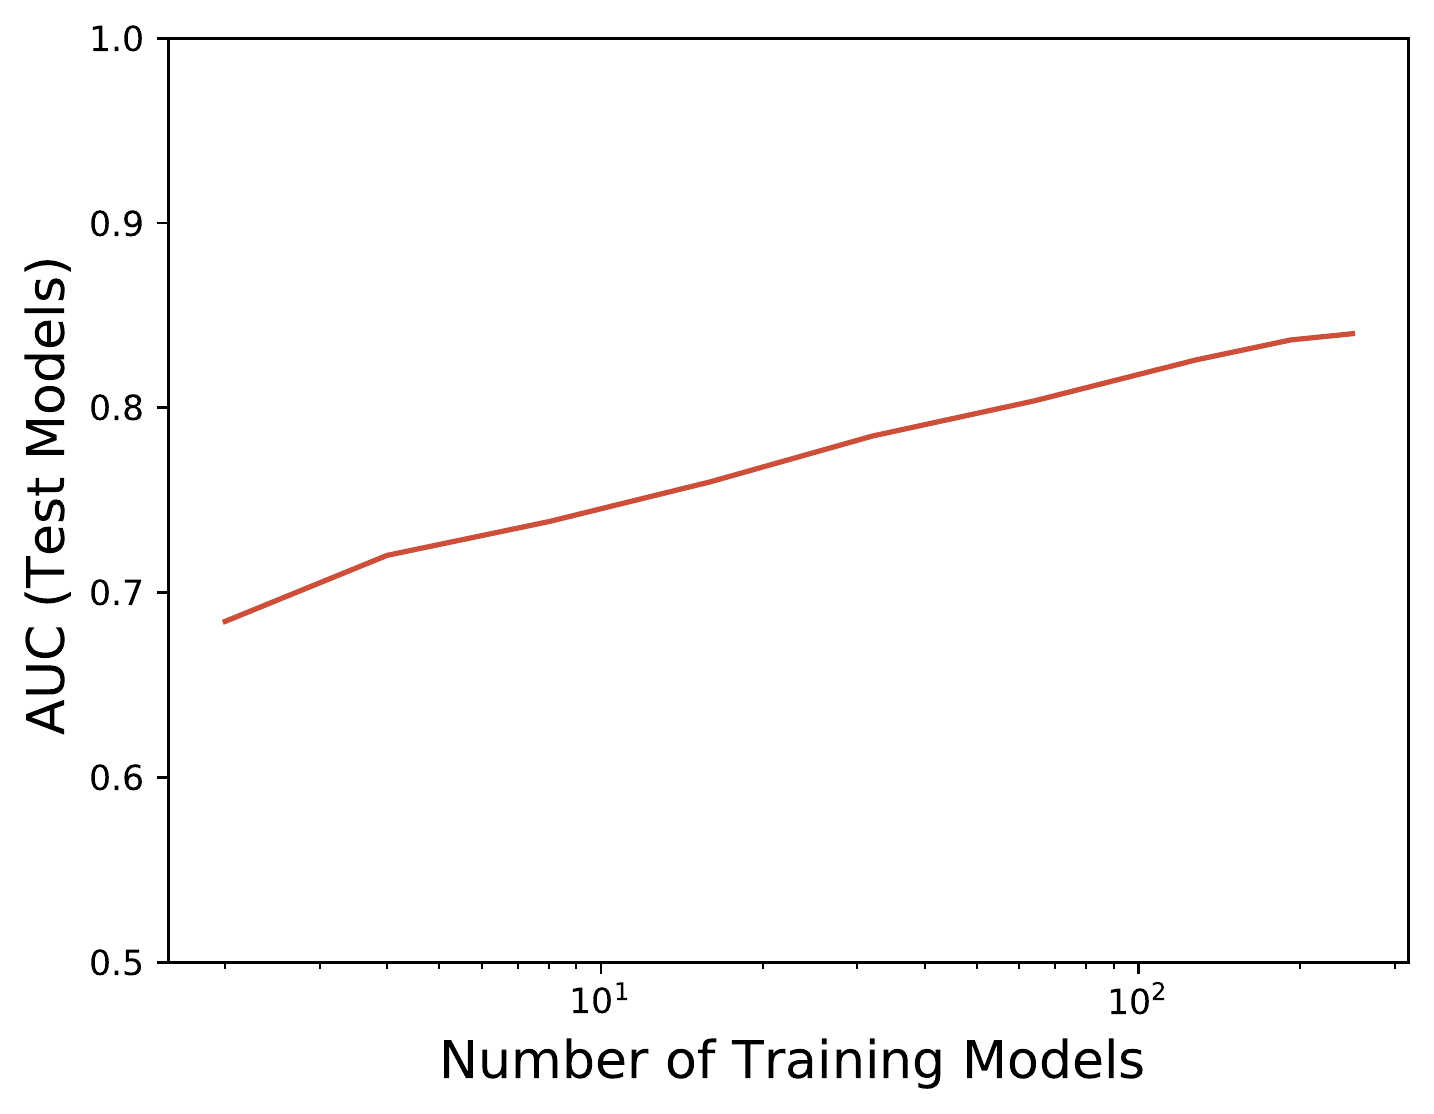}}%
\subfigure[Round 3 ]{%
\label{fig:r3auc_det2}%
\includegraphics[width=.5\textwidth]{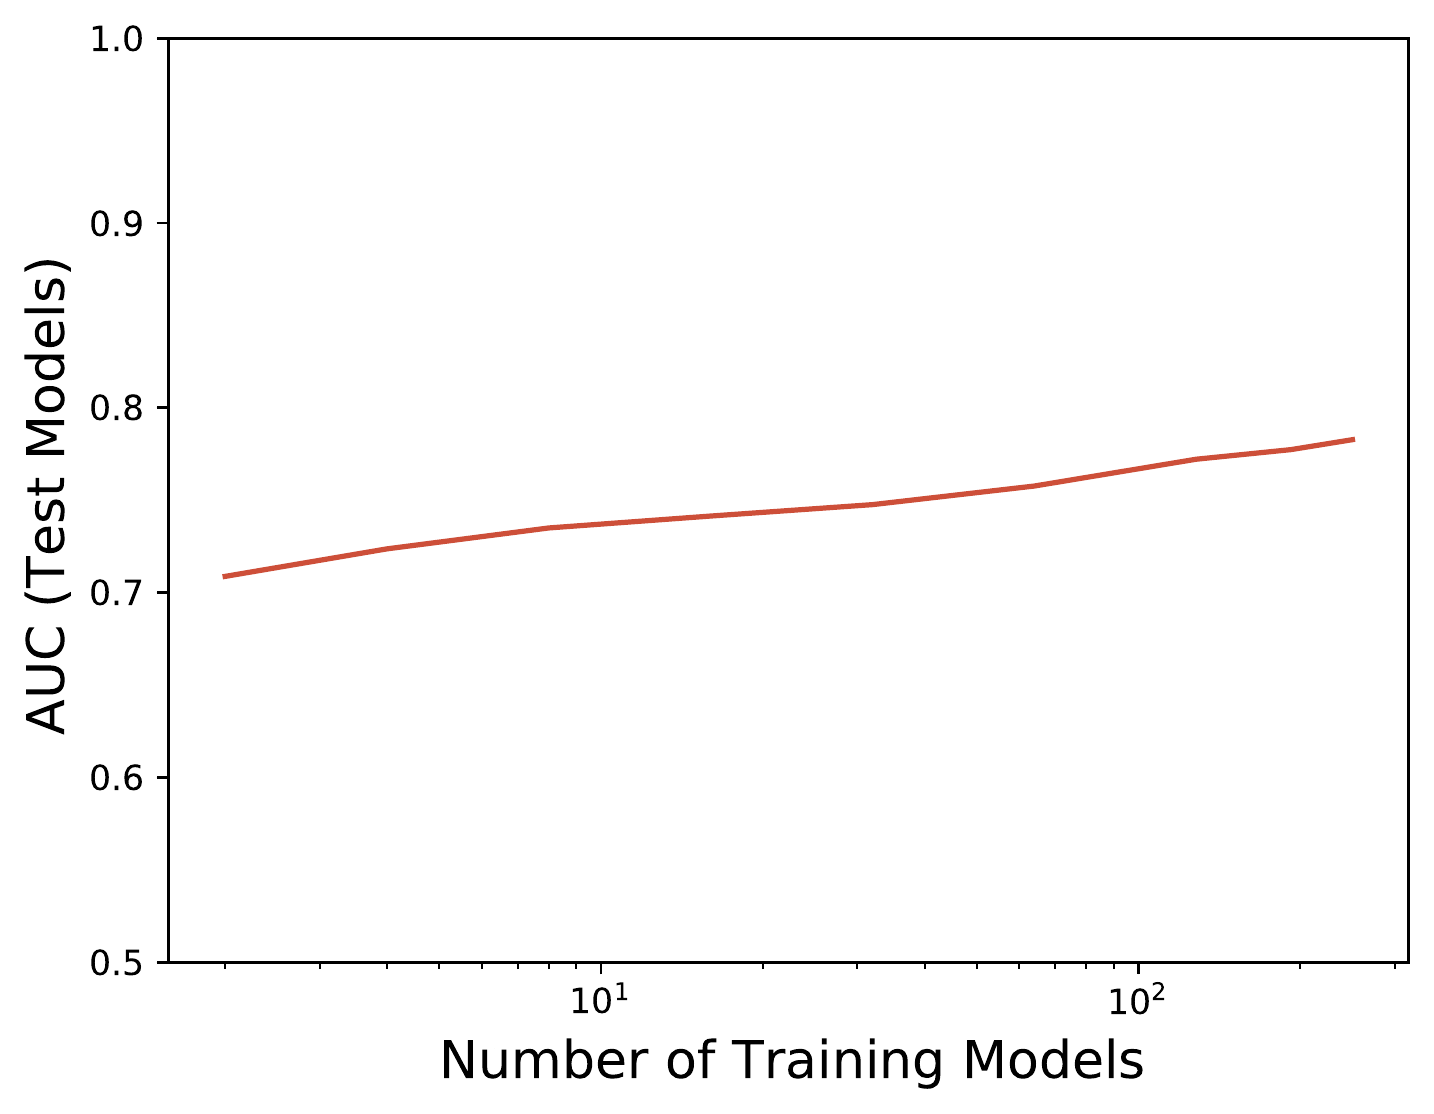}}%
$}
\caption{The AUC for Instagram vs. None corresponding to $\ell_{\infty}$-filter detector}
\end{figure}

\begin{figure}[!htbp]
\resizebox{.98\linewidth}{!}{$
\centering
\subfigure[Round 2]{%
\label{fig:r2ce_det2}%
\includegraphics[width=.5\textwidth]{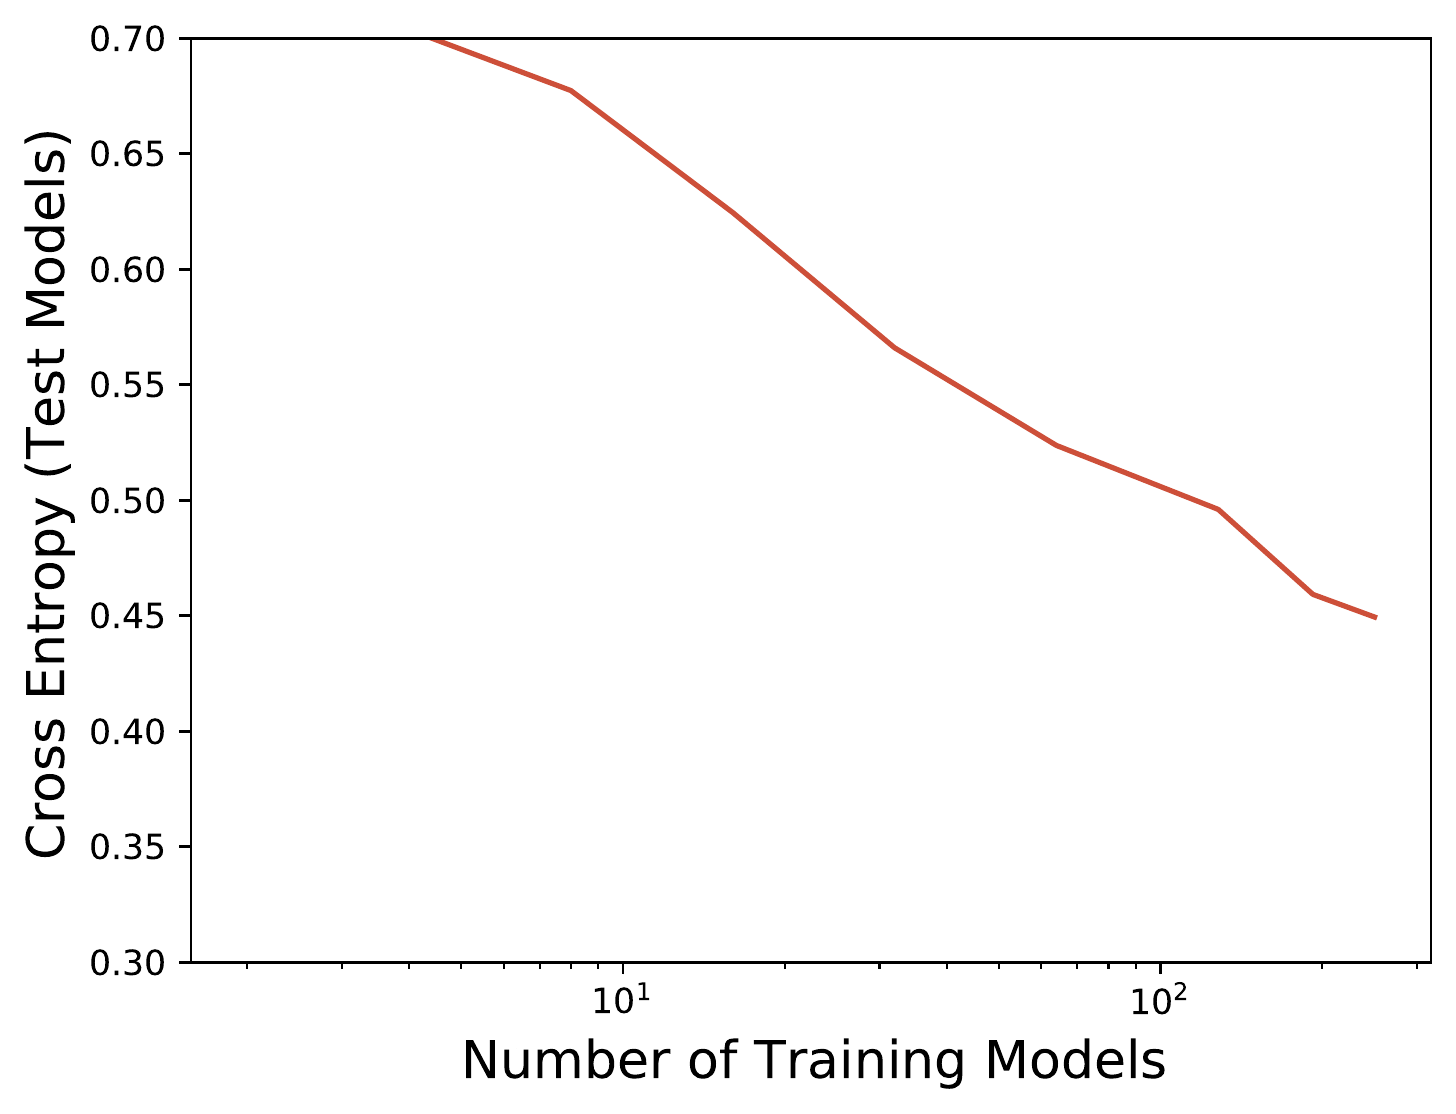}}%
\subfigure[Round 3 ]{%
\label{fig:r3ce_det2}%
\includegraphics[width=.5\textwidth]{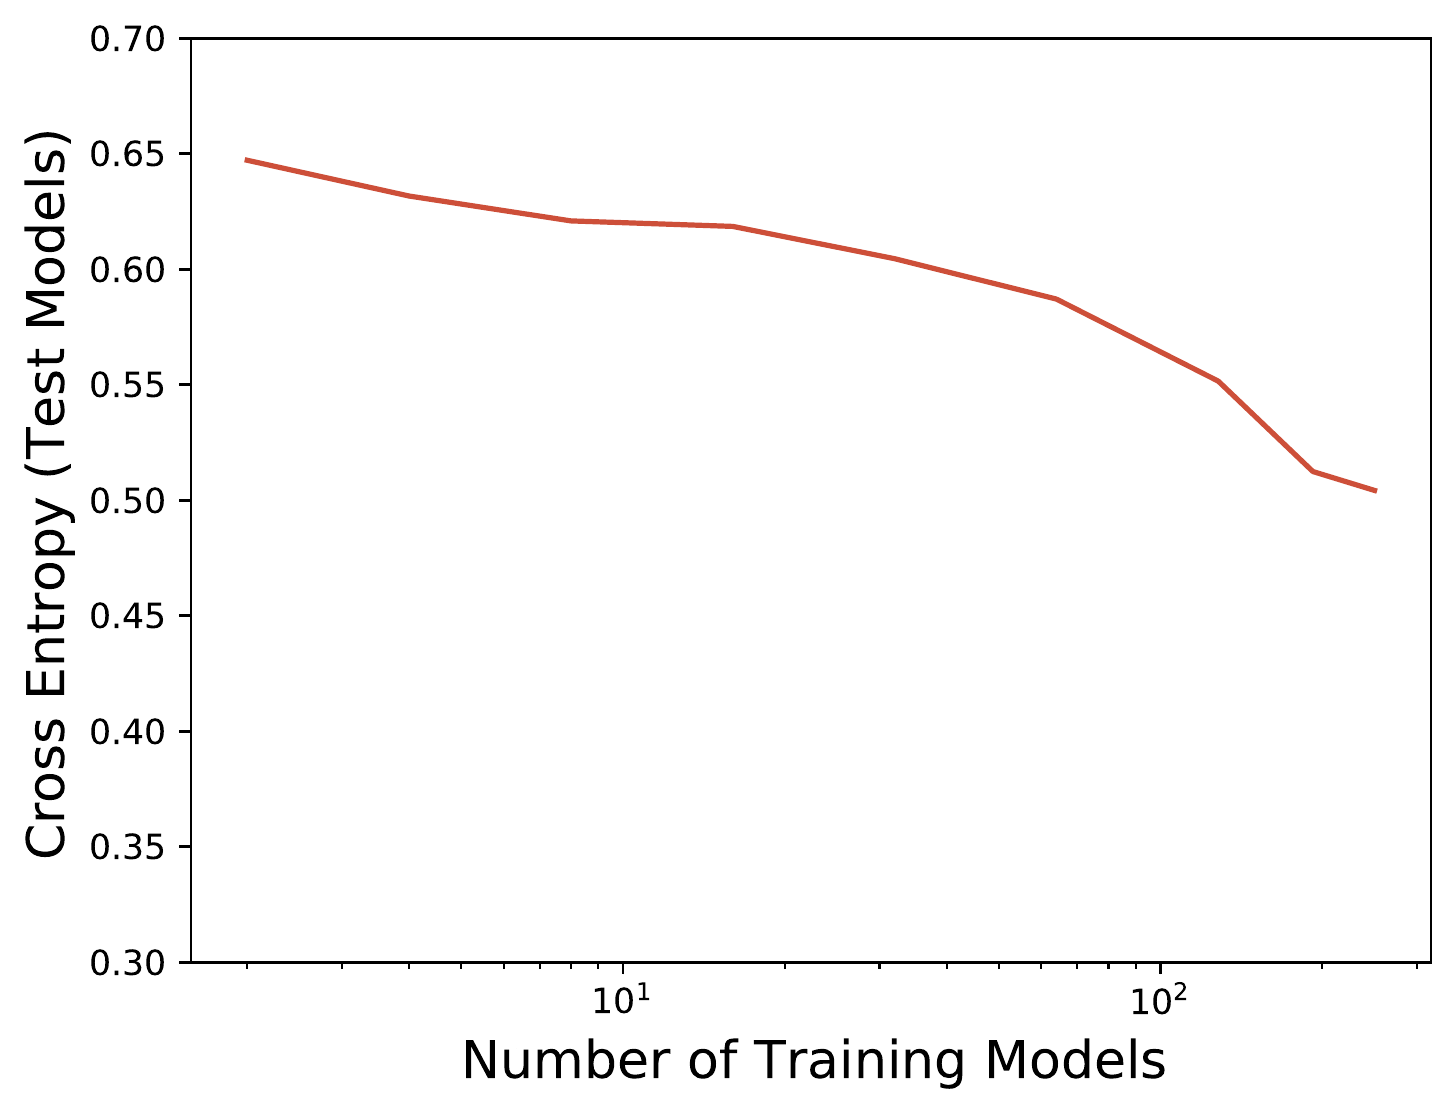}}%
$}
\caption{The CE for Instagram vs. None corresponding to $\ell_{\infty}$-filter detector}
\end{figure}
Figures \ref{fig:r2auc_det2} and \ref{fig:r2ce_det2} show how the number of training models impacts the top-level metric, for the $\ell_{\infty}$ filter detector,  in round 2. Similar, Figures \ref{fig:r3auc_det2} and \ref{fig:r3ce_det2} show how the number of training models impacts the top-level metric, for the $\ell_{\infty}$  filter detector,  in round 3.

 %%%%%%%%%%%%%
%Detector 3
%%%%%%%%%%%%
\begin{figure}[!htbp]
\resizebox{.98\linewidth}{!}{$
\centering
\subfigure[Round 2]{%
\label{fig:r2auc_det3}%
\includegraphics[width=.5\textwidth]{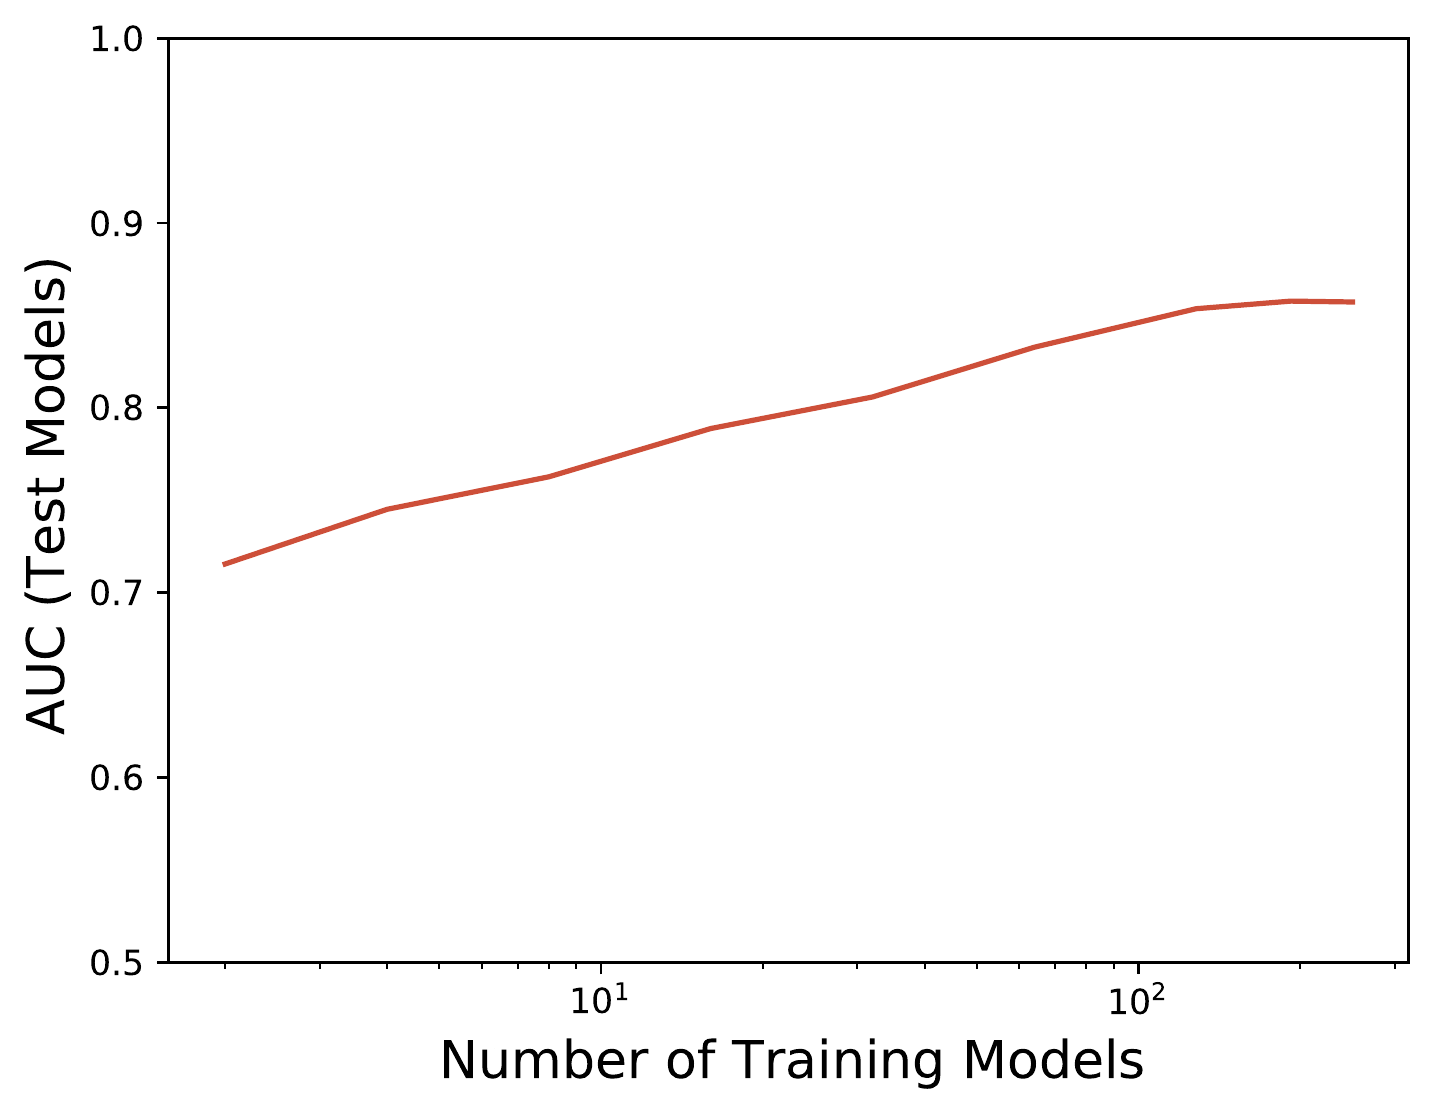}}%
\subfigure[Round 3 ]{%
\label{fig:r2ce_det3}%
\includegraphics[width=.5\textwidth]{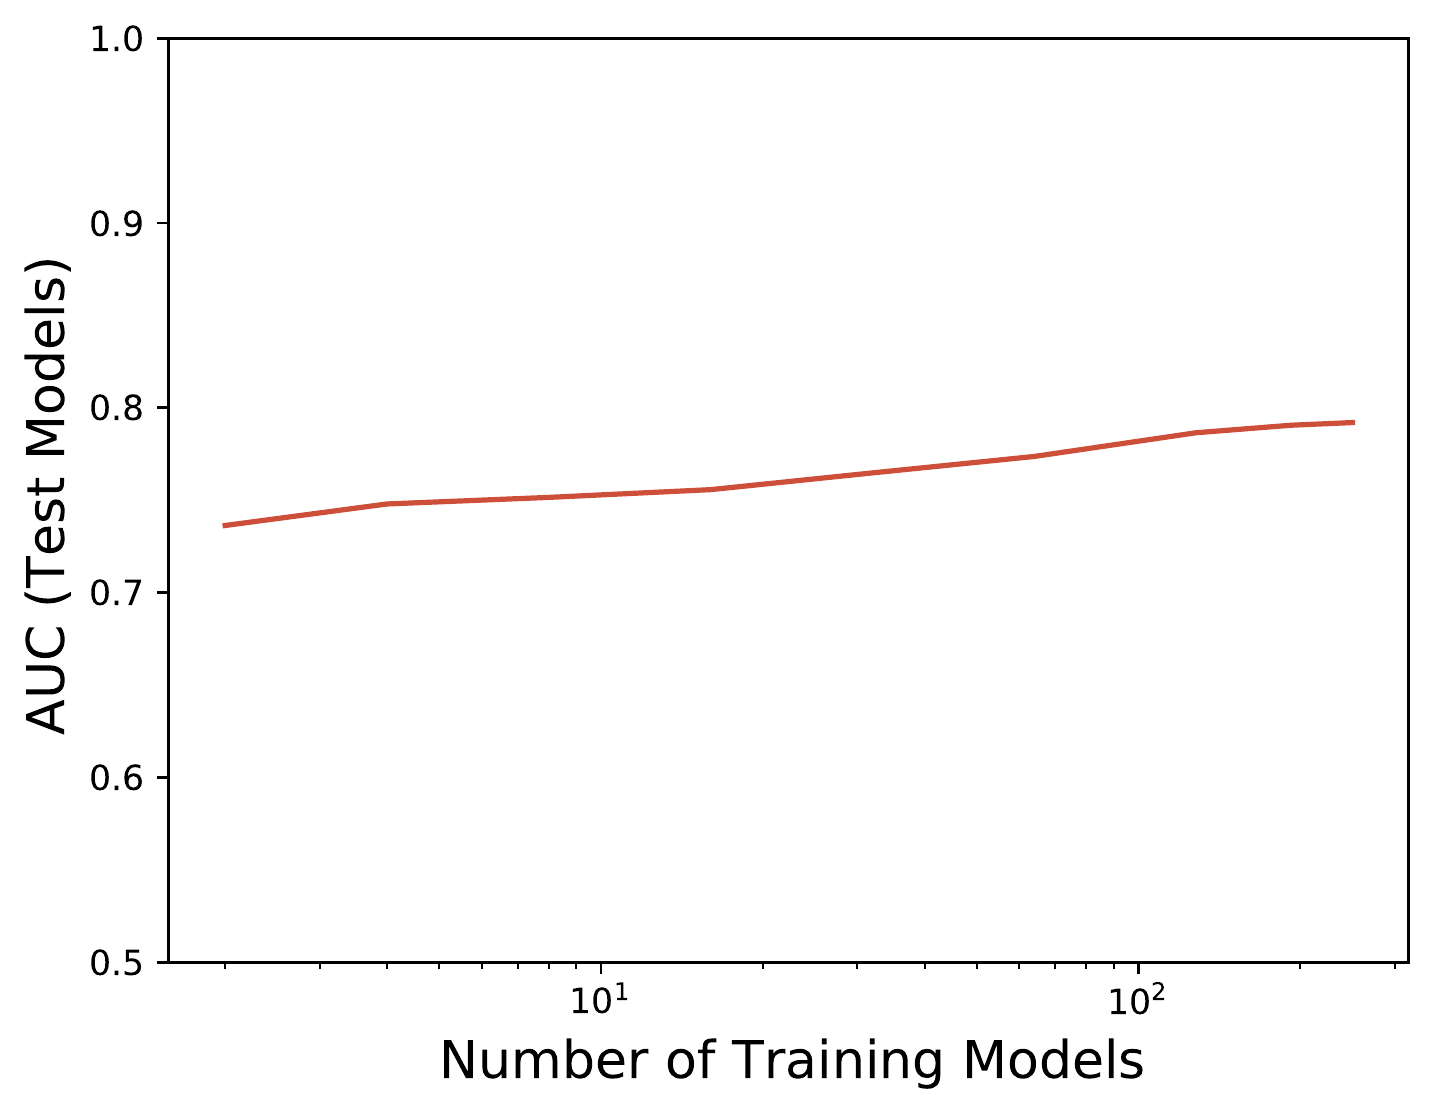}}%
$ }
\caption{The AUC for Instagram vs. None corresponding to $\ell_2$-filter and $\ell_{\infty}$-filter detector}
\end{figure}

\begin{figure}[!htbp]
\resizebox{.98\linewidth}{!}{$
\centering
\subfigure[Round 2]{%
\label{fig:r3auc_det3}%
\includegraphics[width=.5\textwidth]{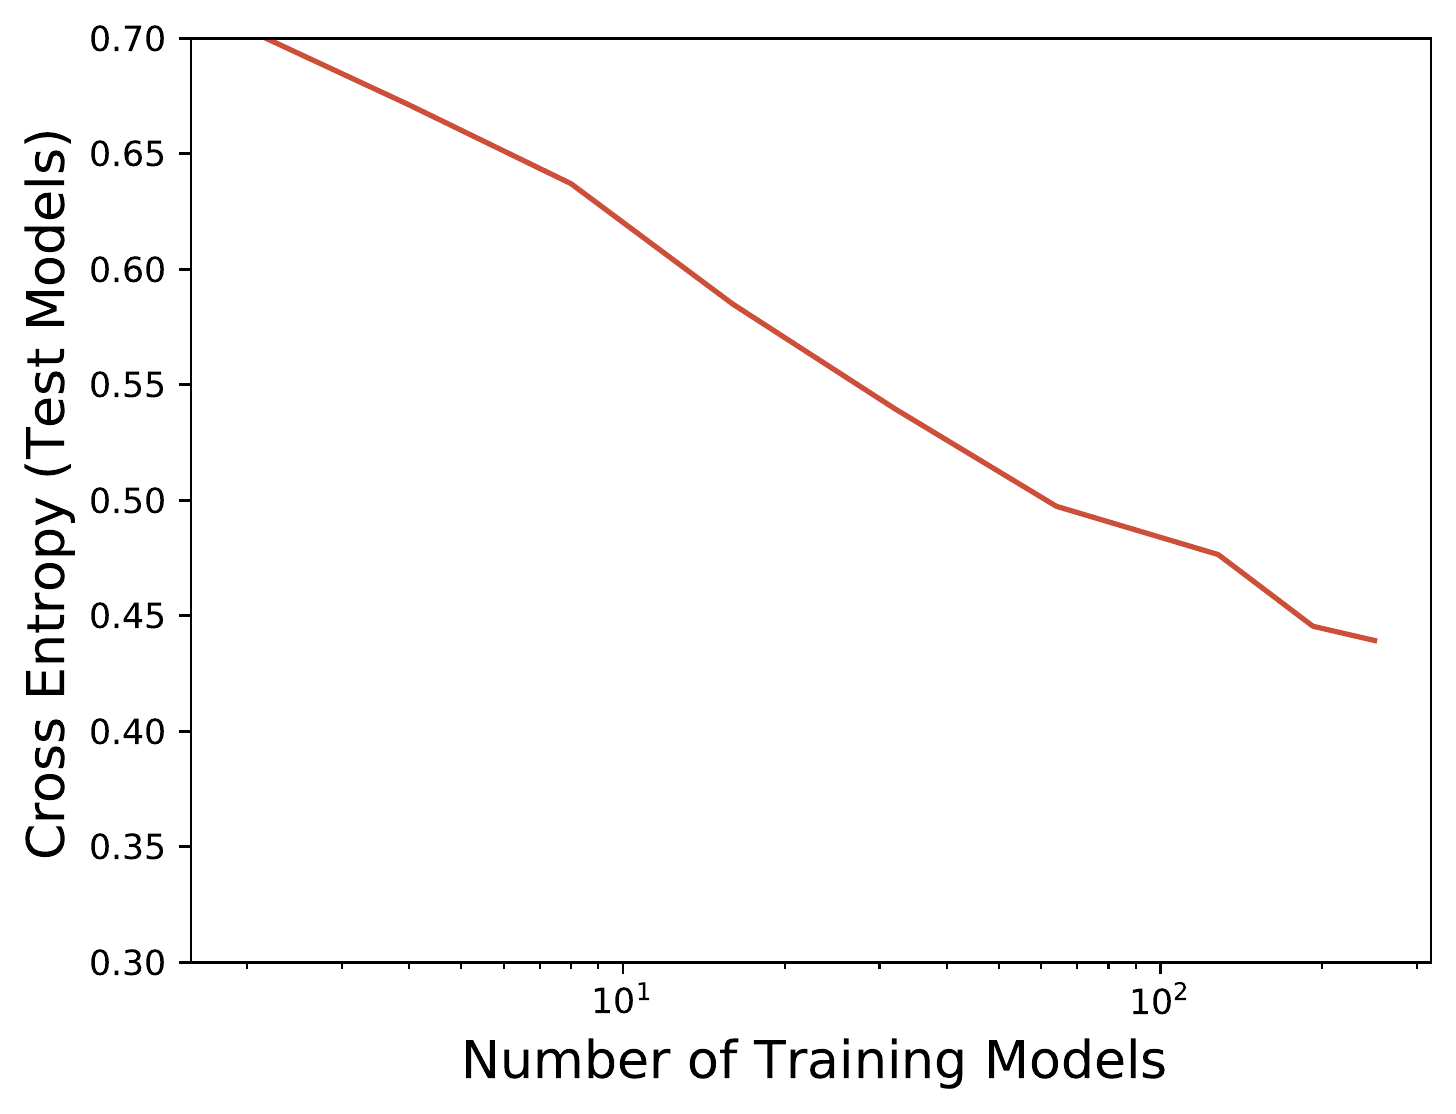}}%
\subfigure[Round 3 ]{%
\label{fig:r3ce_det3}%
\includegraphics[width=.5\textwidth]{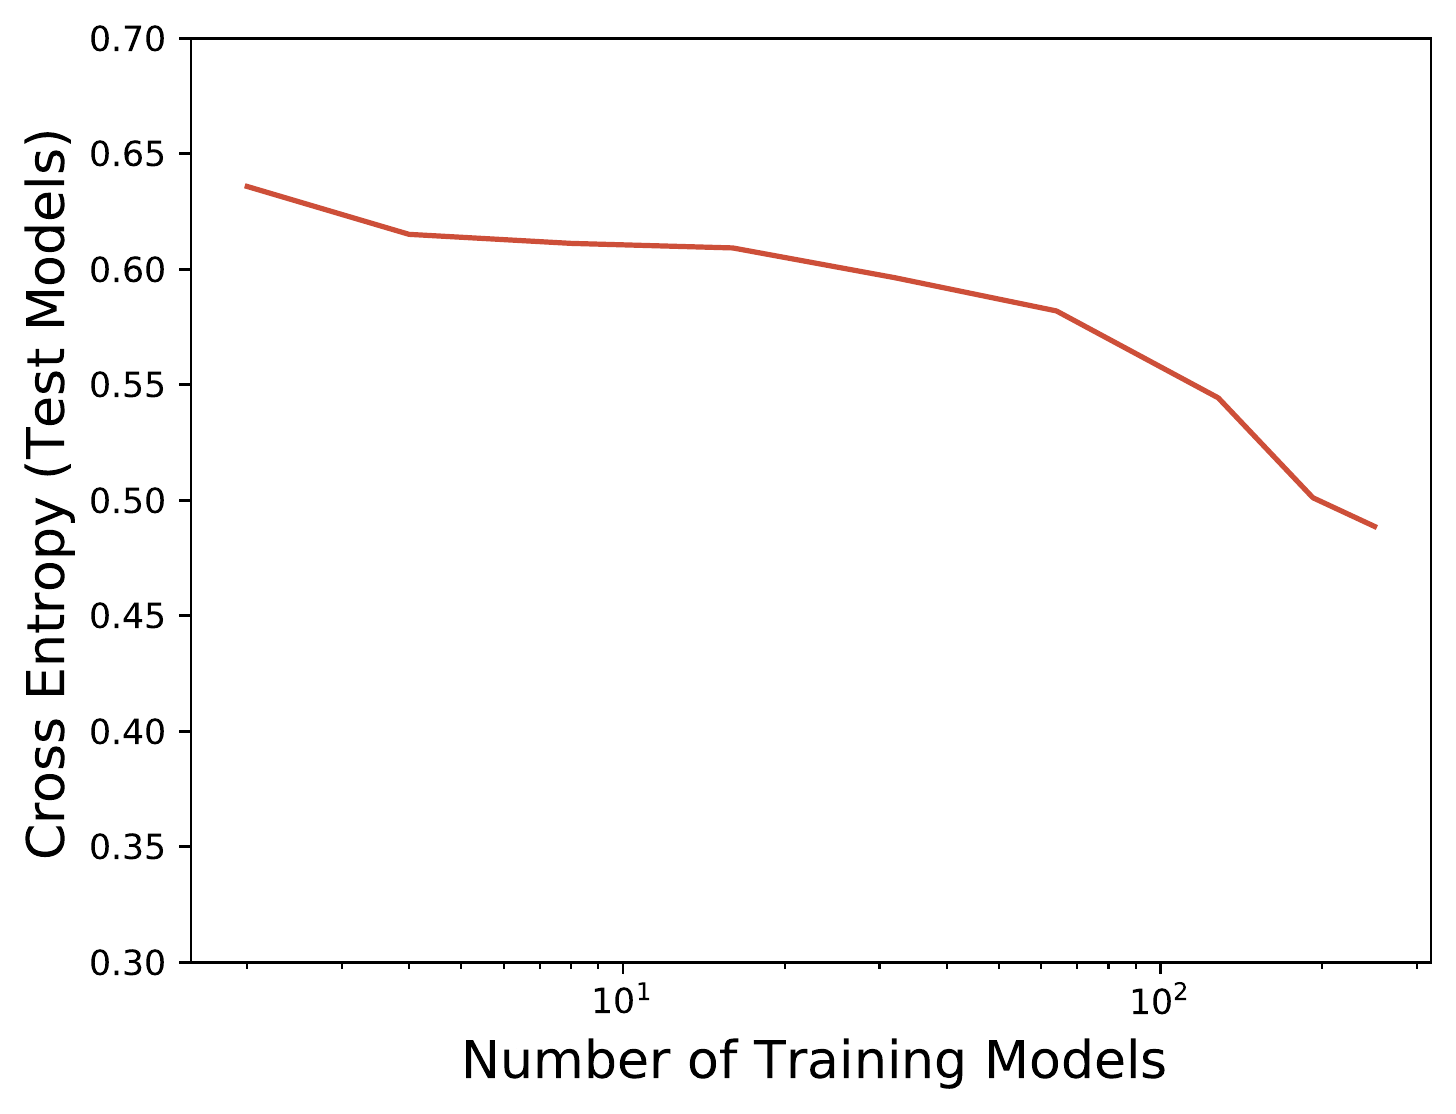}}%
$}
\caption{The CE for Instagram vs. None corresponding to $\ell_2$-filter and $\ell_{\infty}$-filter detector}
\end{figure}
Figures \ref{fig:r2auc_det3} and \ref{fig:r2ce_det3} show how the number of training models impacts the top-level metric, for the $\ell_{2}$ and $\ell_{\infty}$ filter detector,  in round 2. Similar, Figures \ref{fig:r3auc_det3} and \ref{fig:r3ce_det3} show how the number of training models impacts the top-level metric, for the $\ell_{2}$ and $\ell_{\infty}$  filter detector,  in round 3.

 %%%%%%%%%%%%%
%Detector 4
%%%%%%%%%%%%
\begin{figure}[!htbp]
\resizebox{.97\linewidth}{!}{$
\centering
\subfigure[Round 2]{%
\label{fig:r2auc_det4}%
\includegraphics[width=.5\textwidth]{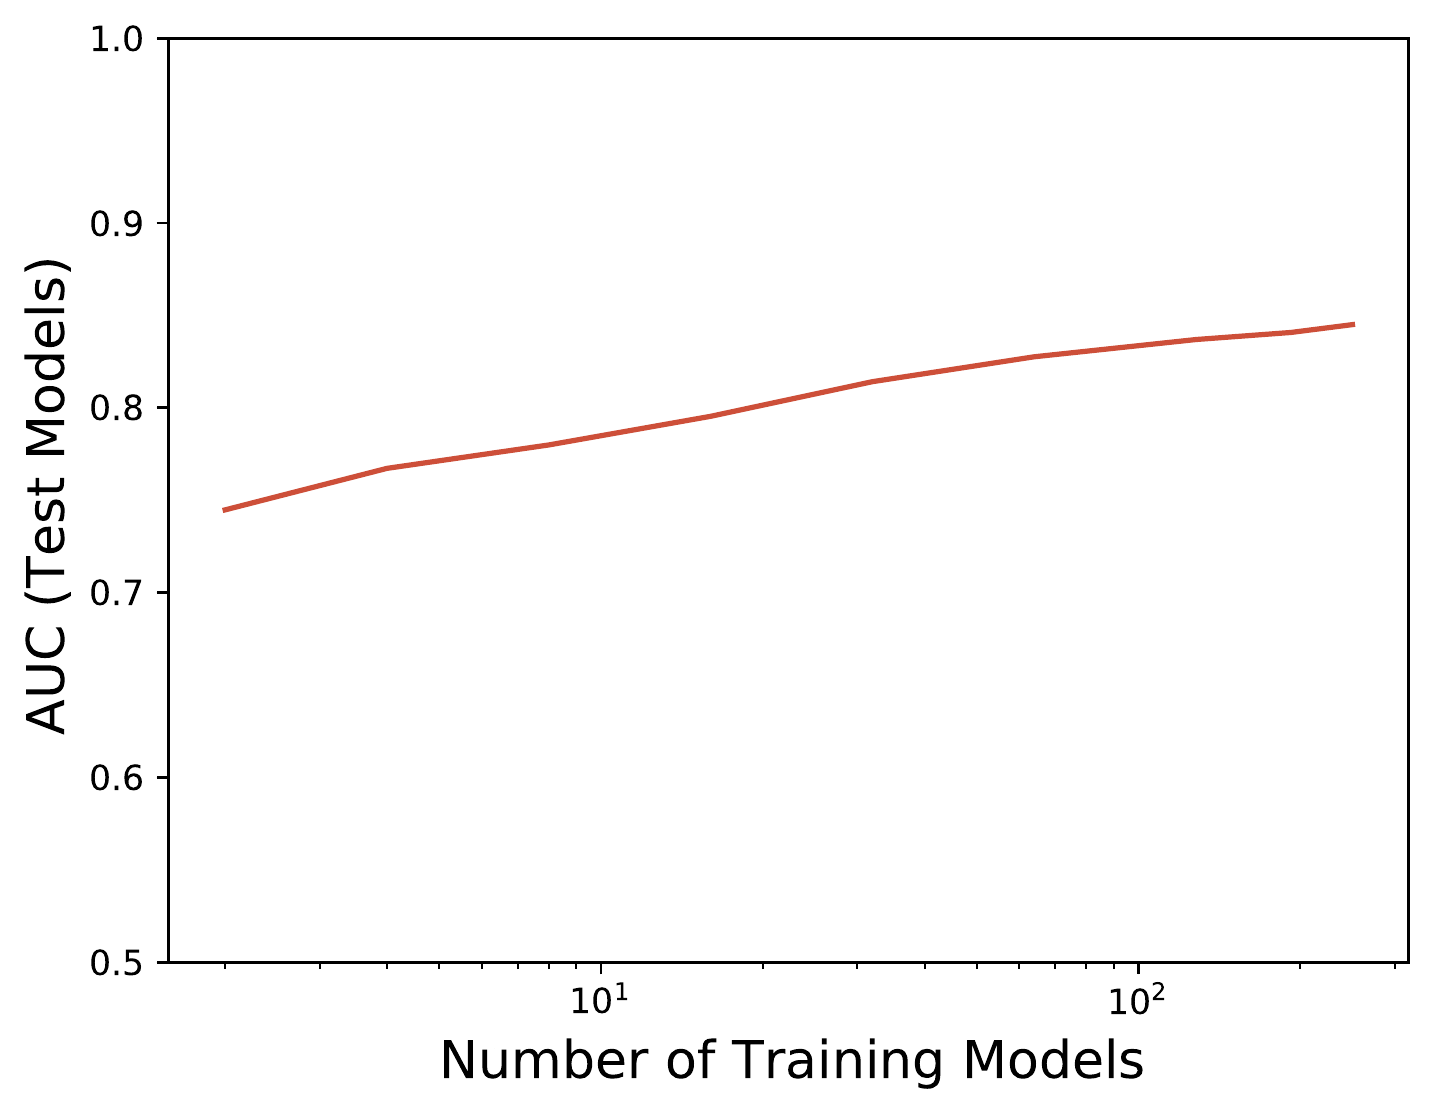}}%
\subfigure[Round 3 ]{%
\label{fig:r3auc_det4}%
\includegraphics[width=.5\textwidth]{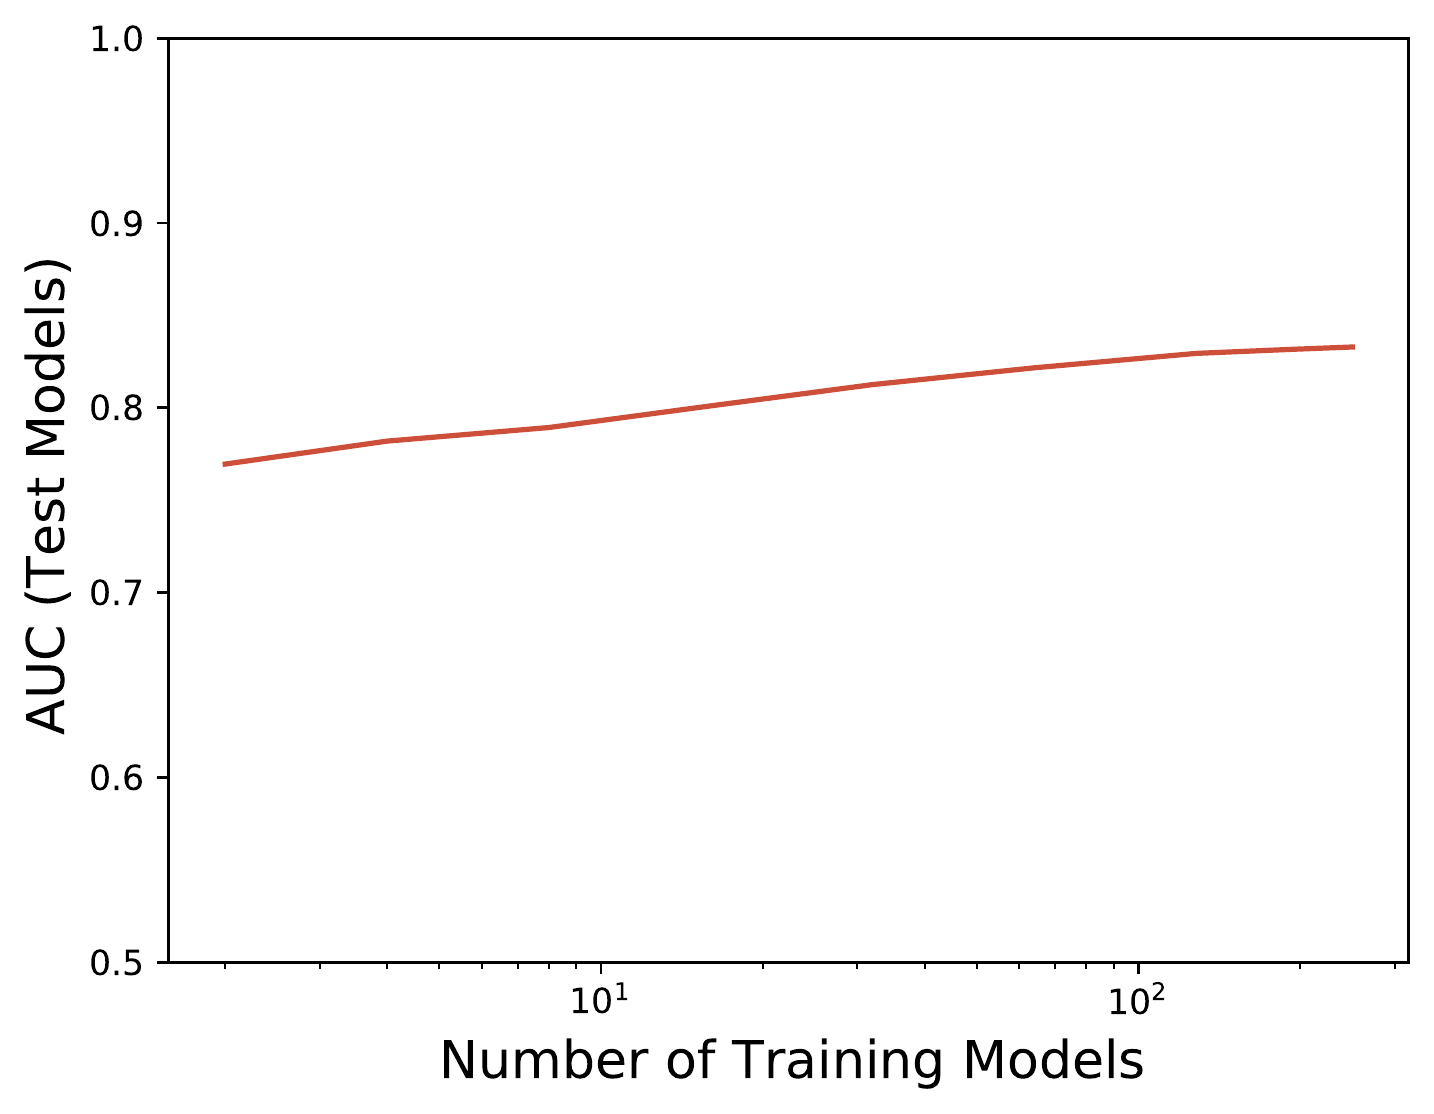}}%
$ }
\caption{The AUC for Instagram vs. None corresponding to $\ell_1$-filter, $\ell_2$-filter, and $\ell_{\infty}$-filter}
\end{figure}

\begin{figure}[!htbp]
\resizebox{.97\linewidth}{!}{$
\centering
\subfigure[Round 2]{%
\label{fig:r2ce_det4}%
\includegraphics[width=.5\textwidth]{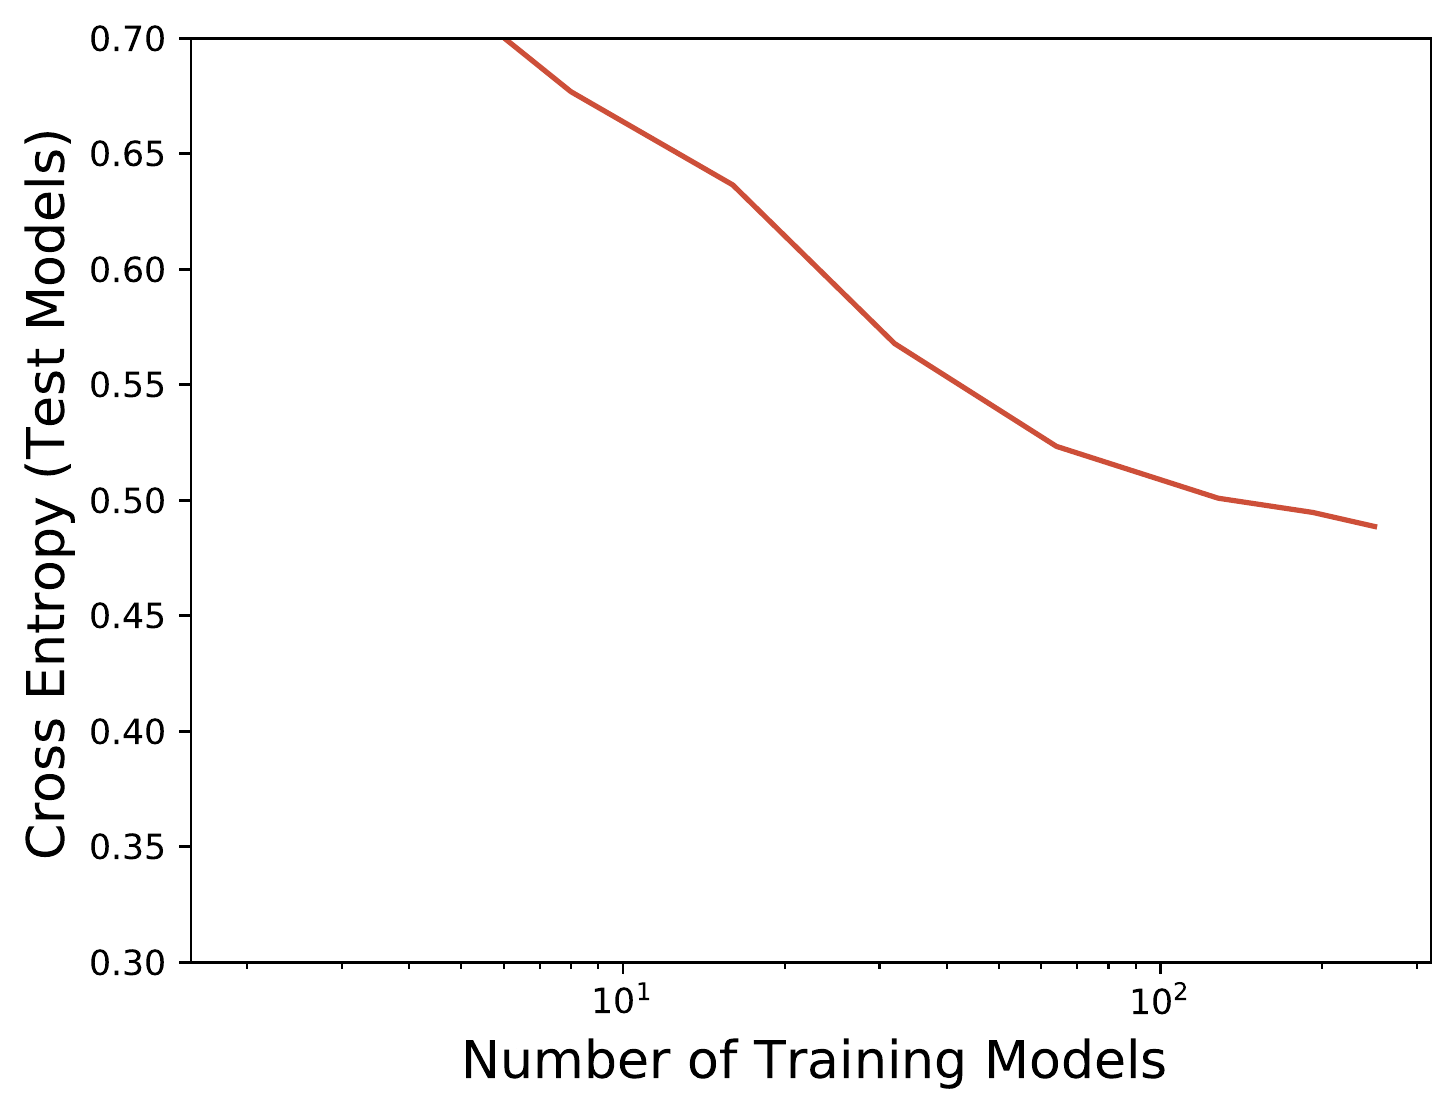}}%
\subfigure[Round 3 ]{%
\label{fig:r3ce_det4}%
\includegraphics[width=.5\textwidth]{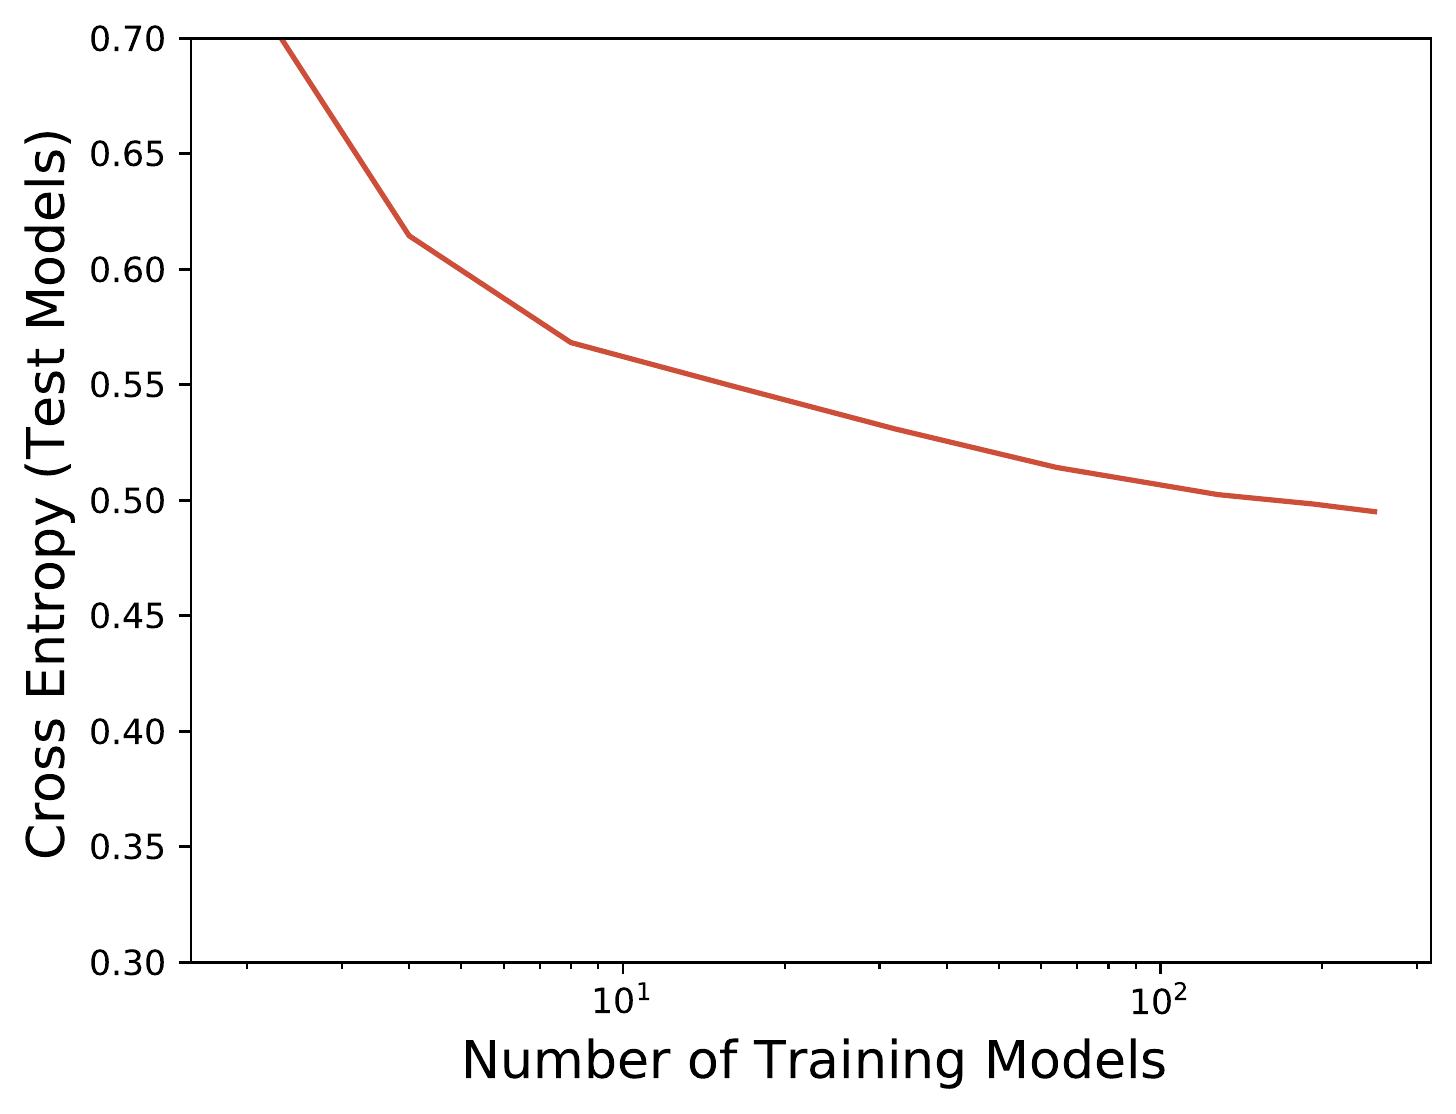}}%
$ }
\caption{The CE for Instagram vs. None corresponding to $\ell_1$-filter, $\ell_2$-filter, and $\ell_{\infty}$-filter detector}
\end{figure}
Figures \ref{fig:r2auc_det4} and \ref{fig:r2ce_det4} show how the number of training models impacts the top-level metric, for the $\ell_{1}$, $\ell_{2}$ and $\ell_{\infty}$ filter detector,  in round 2. Similar, Figures \ref{fig:r3auc_det4} and \ref{fig:r3ce_det4} show how the number of training models impacts the top-level metric, for the $\ell_{1}$, $\ell_{2}$ and $\ell_{\infty}$  filter detector,  in round 3.
% \section{Implementation Details}
